# Supplementary material for: Towards the determination of the dimension of the critical surface in asymptotically safe gravity
Source: arXiv:2004.04126 ancillary file (2020-10-08)
Supplement: Supplementary file 1 [file supplement.pdf]

KU-TP 075-2
July 27, 2020

# Supplementary material – Derivation of beta functions from FRGE with anomalous dimensions


Kevin Falls,[a,b,1] Nobuyoshi Ohta,[c,2] and Roberto Percacci[a,b,3]

[a] *International School for Advanced Studies, via Bonomea 265, 34136 Trieste, Italy*
[b] *INFN, Sezione di Trieste, Italy*
[c] *Department of Physics, Kindai University, Higashi-Osaka, Osaka 577-8502, Japan*


## 1 Definitions

Here we give technical details of the derivation of the FRGE. We use type I cutoff and use RG machine as discussed in [1,2]. We have

$$\begin{aligned}\dot\Gamma_k &= \frac{1}{2}\mathrm{Tr}\frac{\partial_t[KR_k(\Delta^2)]}{K[\mathcal{H}+R_k(\Delta^2)]} - \mathrm{Tr}\frac{\partial_t[Z_{gh}\mathcal{R}_k(\Delta)]}{Z_{gh}[\Delta_{gh}+\mathcal{R}_k(\Delta)]} - \frac{1}{2}\mathrm{Tr}\frac{\partial_t[Z_b\mathcal{R}_k(\Delta)]}{Z_b[Y+\mathcal{R}_k(\Delta)]}\\ &= \frac{1}{2}\mathrm{Tr}\frac{\partial_t R_k(\Delta^2)+\eta_K R_k(\Delta^2)}{\mathcal{H}+R_k(\Delta^2)} - \mathrm{Tr}\frac{\partial_t R_k(\Delta)+\eta_{gh}R_k(\Delta)}{\Delta_{gh}+\mathcal{R}_k(\Delta)} - \frac{1}{2}\mathrm{Tr}\frac{\partial_t R_k(\Delta)+\eta_b R_k(\Delta)}{Y+\mathcal{R}_k(\Delta)},\\ &\equiv T^{\mathrm{grav}}+T^{\mathrm{c}}+T^{\mathrm{b}},\end{aligned} \tag{1.1}$$

where

$$\mathcal{H} = \Delta^2 + V_{\rho\lambda}\bar\nabla^\rho\bar\nabla^\lambda + U, \tag{1.2}$$

$$(\Delta_{gh})_{\mu\nu} = \Delta\bar g_{\mu\nu} - \frac{1-2\omega}{2(1+\omega)}\bar\nabla_\mu\bar\nabla_\nu - \bar R_{\mu\nu},\quad Y_{\mu\nu} = \Delta\bar g_{\mu\nu} + \frac{1-2\omega}{3}\bar\nabla_\mu\bar\nabla_\nu + \bar R_{\mu\nu}, \tag{1.3}$$

and we have introduced the wave function renormalization factors $Z_{gh}$ and $Z_b$, and defined the anomalous dimensions

$$\eta_K = K^{-1}\frac{dK}{dt},\qquad \eta_{gh} = \frac{1}{Z_{gh}}\frac{dZ_{gh}}{dt},\qquad \eta_b = \frac{1}{Z_b}\frac{dZ_b}{dt}, \tag{1.4}$$

in terms of the coefficient

$$(K)_{\mu\nu,\alpha\beta} = \frac{\beta+4\gamma}{4}\Big(\bar g_{\mu\alpha}\bar g_{\nu\beta} + \frac{4\alpha+\beta}{4(\gamma-\alpha)}\bar g_{\mu\nu}\bar g_{\alpha\beta}\Big),\quad (K^{-1})_{\mu\nu}{}^{\alpha\beta} = \frac{4}{\beta+4\gamma}(\delta_{\mu\nu}{}^{\alpha\beta} - \Omega\bar g_{\mu\nu}\bar g^{\alpha\beta}), \tag{1.5}$$

Note that $\eta_K$ is a tensor. We have

$$\eta_K = \eta_1\mathbf{1} + \eta_P\mathbb{P}, \tag{1.6}$$

where

$$\eta_1 = \frac{\dot\beta+4\dot\gamma}{\beta+4\gamma},\qquad \eta_P = \frac{(4\gamma+\beta)\dot\alpha}{(\gamma-\alpha)(3\alpha+\beta+\gamma)} + \frac{\dot\beta}{(3\alpha+\beta+\gamma)} - \frac{(4\alpha+\beta)\dot\gamma}{(\gamma-\alpha)(3\alpha+\beta+\gamma)}\ , \tag{1.7}$$


[1] e-mail address: kfalls@sissa.it
[2] e-mail address: ohtan@phys.kindai.ac.jp
[3] e-mail address: percacci@sissa.it

and the identity in the space of symmetric tensor $\hat{\mathbf{1}}$ and the projector $\mathbb{P}$ are defined by

$$\hat{\mathbf{1}}_{\mu\nu,\alpha\beta} \equiv \delta_{\mu\nu,\alpha\beta} = \frac{1}{2}(\bar{g}_{\mu\alpha}\bar{g}_{\nu\beta} + \bar{g}_{\mu\beta}\bar{g}_{\nu\alpha}), \quad \mathbb{P}^{\mu\nu}{}_{\rho\sigma} \equiv P^{\mu\nu}{}_{\rho\sigma} = \frac{1}{4}\bar{g}^{\mu\nu}\bar{g}_{\rho\sigma} \ . \tag{1.8}$$

The type I cutoff is

$$R_k(\Delta^2) = (k^4 - \Delta^2)\theta(k^4 - \Delta^2), \tag{1.9}$$

and we define as usual

$$P_k(\Delta^2) = \Delta^2 + R_k(\Delta^2) = k^4\theta(k^4 - \Delta^2). \tag{1.10}$$

The tensors $U$ and $V$ are [3]

$$\begin{aligned}(U)_{\mu\nu,\alpha\beta} \;=\; & \frac{4}{\beta+4\gamma}\Bigg[\frac{3}{2}\gamma\bar{g}_{\nu\beta}\bar{R}_{\mu}{}^{\rho\lambda\sigma}\bar{R}_{\alpha\rho\lambda\sigma} - \gamma\bar{R}^{\lambda}{}_{\alpha\mu}{}^{\rho}\bar{R}_{\lambda\nu\beta\rho} + 4\gamma\bar{R}_{\rho\alpha\mu\lambda}\bar{R}_{\nu\beta}{}^{\rho\lambda} \\ & -3\gamma(\bar{R}^{\sigma}_{\mu}\bar{R}_{\sigma\alpha\nu\beta} + \bar{R}^{\sigma}_{\alpha}\bar{R}_{\sigma\mu\beta\nu}) + \Big(\frac{\beta}{2}+\gamma\Big)\bar{R}_{\mu\alpha}\bar{R}_{\nu\beta} - \frac{\gamma}{2}\bar{g}_{\alpha\beta}\bar{R}_{\mu\rho\lambda\sigma}\bar{R}_{\nu}{}^{\rho\lambda\sigma} \\ & +\frac{1}{4}S^2(\Omega_1\bar{g}_{\mu\nu}\bar{g}_{\alpha\beta} - \bar{g}_{\mu\alpha}\bar{g}_{\nu\beta}) + \Big(\frac{\alpha}{2}\bar{R} - \frac{Z_N}{4}\Big)(\bar{R}_{\mu\alpha\nu\beta} + 3\bar{g}_{\nu\beta}\bar{R}_{\mu\alpha} - \bar{g}_{\alpha\beta}\bar{R}_{\mu\nu}) \\ & +\Big(\frac{5}{2}\beta+4\gamma\Big)\bar{g}_{\nu\beta}\bar{R}_{\mu\sigma}\bar{R}^{\sigma}_{\alpha} + (\beta+5\gamma)\bar{R}_{\rho\mu\lambda\nu}\bar{R}^{\rho}{}_{\alpha}{}^{\lambda}{}_{\beta} - \frac{\beta}{2}\bar{g}_{\alpha\beta}\bar{R}_{\mu\sigma}\bar{R}^{\sigma}_{\nu} \\ & -\gamma\Omega_1\bar{g}_{\mu\nu}\bar{R}_{\alpha\rho\lambda\sigma}\bar{R}_{\beta}{}^{\rho\lambda\sigma} - \beta\Omega_1\bar{g}_{\mu\nu}\bar{R}_{\alpha\sigma}\bar{R}^{\sigma}_{\beta} + \alpha\bar{R}_{\mu\nu}\bar{R}_{\alpha\beta} + \Big(Z_N\Omega_3 - \alpha\Omega_1\bar{R}\Big)\bar{g}_{\mu\nu}\bar{R}_{\alpha\beta} \\ & +\frac{Z_N}{4}(\bar{R}-4\Lambda)\Omega\bar{g}_{\mu\nu}\bar{g}_{\alpha\beta} - (\beta+4\gamma)\bar{g}_{\nu\beta}\bar{R}^{\rho\lambda}\bar{R}_{\mu\rho\alpha\lambda}\Bigg],\end{aligned} \tag{1.11}$$

where we have defined

$$S^2 = \alpha\bar{R}^2 + \beta\bar{R}^2_{\mu\nu} + \gamma\bar{R}^2_{\mu\nu\rho\lambda} - Z_N(\bar{R} - 2\Lambda), \tag{1.12}$$

$$\Omega = \frac{4\alpha+\beta}{\Sigma}, \quad \Omega_1 = \frac{10\alpha+3\beta+2\gamma}{\Sigma}, \quad \Omega_3 = \frac{3\alpha+\beta+\gamma}{\Sigma}, \quad \Sigma \equiv 4(3\alpha+\beta+\gamma). \tag{1.13}$$

$$V^{\rho\lambda} = \frac{4}{\beta+4\gamma}\sum_{i=1}^{20} b_i\mathbf{k}_i, \tag{1.14}$$

where

$$\begin{aligned}&\mathbf{k}_1 = \bar{g}_{\nu\beta}\bar{g}^{\rho\lambda}\bar{R}_{\mu\alpha}, \quad \mathbf{k}_2 = \delta_{\mu\nu,\alpha\beta}\bar{g}^{\rho\lambda}, \quad \mathbf{k}_3 = \bar{g}^{\rho\lambda}\bar{R}_{\mu\alpha\nu\beta}, \quad \mathbf{k}_4 = \delta_{\nu\beta}{}^{\rho\lambda}\bar{R}_{\mu\alpha}, \\ &\mathbf{k}_5 = \delta_{\nu\beta}{}^{\rho\lambda}\bar{g}_{\mu\alpha}, \quad \mathbf{k}_6 = \delta_{\mu\nu,\alpha\beta}\bar{R}^{\rho\lambda}, \quad \mathbf{k}_7 = \frac{1}{2}(\delta^{(\rho}_{\nu}\bar{R}^{\lambda)}{}_{\alpha\beta\mu} + \delta^{(\rho}_{\beta}\bar{R}^{\lambda)}{}_{\mu\nu\alpha}), \\ &\mathbf{k}_8 = \bar{g}_{\nu\beta}\delta^{(\rho}_{(\mu}\bar{R}^{\lambda)}_{\alpha)}, \quad \mathbf{k}_9 = \bar{g}_{\nu\beta}\bar{R}_{(\alpha}{}^{\rho\lambda}{}_{\mu)}, \quad \mathbf{k}_{10} = \frac{1}{2}(\delta_{\alpha\beta}{}^{\rho\lambda}\bar{R}_{\mu\nu} + \delta_{\mu\nu}{}^{\rho\lambda}\bar{R}_{\alpha\beta}), \\ &\mathbf{k}_{11} = \bar{g}_{\mu\nu}\bar{R}_{\alpha}{}^{\rho\lambda}{}_{\beta}, \quad \mathbf{k}_{12} = \bar{g}_{\alpha\beta}\bar{R}_{\mu}{}^{\rho\lambda}{}_{\nu}, \quad \mathbf{k}_{13} = \bar{g}_{\mu\nu}\bar{g}^{\rho\lambda}\bar{R}_{\alpha\beta}, \quad \mathbf{k}_{14} = \bar{g}_{\alpha\beta}\bar{g}^{\rho\lambda}\bar{R}_{\mu\nu}, \\ &\mathbf{k}_{15} = \bar{g}_{\mu\nu}\delta^{\lambda}_{\alpha}\bar{R}^{\rho}_{\beta}, \quad \mathbf{k}_{16} = \bar{g}_{\alpha\beta}\delta^{\lambda}_{\mu}\bar{R}^{\rho}_{\nu}, \quad \mathbf{k}_{17} = \bar{g}_{\mu\nu}\delta_{\alpha\beta}{}^{\rho\lambda}, \quad \mathbf{k}_{18} = \bar{g}_{\alpha\beta}\delta_{\mu\nu}{}^{\rho\lambda}, \\ &\mathbf{k}_{19} = \bar{g}_{\mu\nu}\bar{g}_{\alpha\beta}\bar{g}^{\rho\lambda}, \quad \mathbf{k}_{20} = \bar{g}_{\mu\nu}\bar{g}_{\alpha\beta}\bar{R}^{\rho\lambda},\end{aligned} \tag{1.15}$$

$$b_1 = -2\gamma, \quad b_2 = \frac{\alpha}{2}\bar{R} - \frac{Z_N}{4}, \quad b_3 = \beta + 3\gamma, \quad b_4 = 2\gamma, \quad b_5 = \frac{Z_N}{2} - \alpha\bar{R},$$
$$b_6 = \frac{\beta}{2} + \gamma, \quad b_7 = -4\gamma, \quad b_8 = -2\beta - 4\gamma, \quad b_9 = -2\gamma, \quad b_{10} = -2\alpha,$$
$$b_{11} = 4\gamma\Omega_3, \quad b_{12} = \gamma, \quad b_{13} = -\beta\Omega_3, \quad b_{14} = \alpha, \quad b_{15} = 2\beta\Omega_3, \quad b_{16} = \frac{\beta}{2},$$
$$b_{17} = 2\alpha\Omega_3\bar{R} - Z_N\frac{\Omega_1 - 2\Omega}{2}, \quad b_{18} = \frac{\alpha}{2}\bar{R} - \frac{Z_N}{4}, \quad b_{19} = -b_{17}, \quad b_{20} = -\beta\Omega_3. \quad (1.16)$$

It should be understood that the indices are symmetrized in $(\mu,\nu),(\alpha,\beta)$ and $(\rho,\lambda)$ in both $U$ and $V$.

In the old result, those terms of non-negative powers of the cutoff $k$ are kept on the rhs, and only asymptotically safe fixed points were found for the dimensionless couplings. It turns out that this overlooks some terms of order $Z_N$. Here we keep all terms up to the first order in $Z_N$ and second order in the curvatures, and we find that the contributions of these terms allow the existence of interacting fixed points for the higher derivative terms.

## 2 Graviton sector with full dependence on $\Lambda$

The kinetic operator has the form

$$\Delta^2 + V + U. \quad (2.1)$$

The graviton contribution to the FRGE is

$$T^{\rm grav} = \frac{1}{2}{\rm Tr}\left[\frac{\partial_t R_k(\Delta^2) + \eta_K R_k(\Delta^2)}{P_k(\Delta^2) + V + U}\right], \quad (2.2)$$

We divide $V$ and $U$ into parts with different powers of curvature

$$V = V_0 + V_1 \; ; \qquad U = U_0 + U_1 + U_2, \quad (2.3)$$

where

$$V_0 \sim Z_N \nabla\nabla \; ; \qquad V_1 \sim R\nabla\nabla, \quad (2.4)$$
$$U_0 \sim \Lambda Z_N \; ; \qquad U_1 \sim Z_N R \; ; \qquad U_2 \sim R^2 \; .$$

It is possible without too much effort to keep the full dependence on $\Lambda$. We will therefore do this and not expand in $U_0$. However we expand in $V_0$, $V_1$, $U_1$ and $U_2$ to second order in R and first order in Z. Thus we write

$$T^{\rm grav} = \frac{1}{2}{\rm Tr}\frac{\partial_t R_k(\Delta^2) + \eta_K R_k(\Delta^2)}{(P_k(\Delta^2) + U_0)\left(1 + \frac{V_0+V_1+U_1+U_2}{P_k(\Delta^2)+U_0}\right)} \quad (2.5)$$
$$= \frac{1}{2}{\rm Tr}\left[\frac{\partial_t R_k(\Delta^2) + \eta_K R_k(\Delta^2)}{P_k(\Delta^2) + U_0}\left(1 - \frac{V_0+V_1+U_1+U_2}{P_k(\Delta^2)+U_0}\right.\right.$$
$$+\frac{V_0+V_1+U_1+U_2}{P_k(\Delta^2)+U_0}\,\frac{V_0+V_1+U_1+U_2}{P_k(\Delta^2)+U_0}$$
$$\left.\left.-\frac{V_0+V_1+U_1+U_2}{P_k(\Delta^2)+U_0}\,\frac{V_0+V_1+U_1+U_2}{P_k(\Delta^2)+U_0}\,\frac{V_0+V_1+U_1+U_2}{P_k(\Delta^2)+U_0} + \cdots\right)\right], \quad (2.6)$$

Here the notation is a bit sloppy, because $V$ does not commute with the function of $\Delta$ in the denominator. Conventionally here and in the following, we assume that

$$\frac{V}{P_k(\Delta^2)+U_0} = \frac{1}{P_k(\Delta^2)+U_0}V.$$

Keeping only terms up to linear order in $Z_N$ we have the general structure:

$$\begin{aligned} T^{\rm grav} &= \frac{1}{2}{\rm Tr}\left[\frac{\partial_t R_k(\Delta^2)+\eta_K R_k(\Delta^2)}{P_k(\Delta^2)+U_0}\left(1-\frac{1}{P_k(\Delta^2)+U_0}(V_0+V_1+U_1+U_2)\right.\right. \\ &+\frac{1}{P_k(\Delta^2)+U_0}V_0\frac{1}{P_k(\Delta^2)+U_0}V_1+\frac{1}{P_k(\Delta^2)+U_0}V_1\frac{1}{P_k(\Delta^2)+U_0}V_0 \\ &\left.\left.+\frac{2V_0U_2}{(P_k(\Delta^2)+U_0)^2}+\frac{V_1^2}{(P_k(\Delta^2)+U_0)^2}+\frac{2V_1U_1}{(P_k(\Delta^2)+U_0)^2}+\frac{3V_0V_1^2}{(P_k(\Delta^2)+U_0)^3}\right)\right] \\ &\equiv T_1+T_2+T_3+T_4+T_5+T_6+T_7+T_8+T_9+T_{10}\ . \end{aligned} \tag{2.7}$$

In the last line, we have not been careful to order the factors because these terms are already of order $R^2$. The terms $T_n$ are ordered as follows:

1. 1 , evaluated below
2. $V_1$ , evaluated below
3. $V_1^2$ , evaluated below
4. $U_2$ , evaluated below
5. $V_0$ , here we need to expand the heat kernel to order $R^2$.
6. $V_0V_1$ , here we need to expand the heat kernel to order $R$.
7. $V_0V_1^2$ , evaluated below
8. $V_0U_2$ , evaluated below
9. $U_1$ , here we need to expand the heat kernel to order $R$
10. $V_1U_1$ , evaluated below

The first four items are of order $Z_N^0$ and reproduce the standard beta functions.

Let us write

$$U_0 = u_1\mathbb{I}+u_P\mathbb{P},$$

where

$$u_1 = -\frac{2Z_N\Lambda}{\beta+4\gamma}\ ; \qquad u_P = \frac{2Z_N\Lambda\, d(2\alpha+\beta+2\gamma)}{(\beta+4\gamma)(4(d-1)\alpha+d\beta+4\gamma)}\ .$$

Following already established procedure we have

$$\begin{aligned} \frac{1}{P_k+U_0} &= \frac{1}{(P_k+u_1)\left(1+\frac{u_P}{P_k+u_1}\mathbb{P}\right)} \\ &= \frac{1}{(P_k+u_1)}\left(\mathbb{I}-\frac{u_P}{P_k+u_1+u_P}\mathbb{P}\right) \\ &\equiv G_1\mathbb{I}+G_P\mathbb{P}, \end{aligned} \tag{2.8}$$

and similarly

$$\begin{aligned}\frac{\dot{R}_k+\eta_K R_k}{P_k+U_0} &= \frac{\dot{R}_k+\eta_1 R_k}{P_k+u_1}\mathbb{I}+\left(\frac{\eta_P R_k}{P_k+u_1}-\frac{u_P(\dot{R}_k+\eta_1 R_k+\eta_P R_k}{(P_k+u_1)(P_k+u_1+u_P)}\right)\mathbb{P}\\ &\equiv M_1\mathbb{I}+M_P\mathbb{P}. \end{aligned}\tag{2.9}$$

When these are inserted in (2.7), one has to pay attention to the order of terms. Even though $\mathbb{P}$ commutes with the Laplacian, it is contracted in specific ways to the indices on $U$ and $V$. In general $\mathbb{P}$ can appear in several positions and these terms are not equal a priori.

In the following traces, we will need the following totally symmetric tensors:

$$\begin{aligned}S_{\mu\nu} &= g_{\mu\nu},\\ S_{\mu\nu\rho\sigma} &= g_{(\mu\nu}g_{\rho\sigma)},\\ S_{\mu\nu\rho\sigma\lambda\tau} &= g_{(\mu\nu}g_{\rho\sigma}g_{\lambda\tau)}. \end{aligned}\tag{2.10}$$

Notation: the traces "Tr" are in the functional space of symmetric tensor fields, the traces "tr" are over the finite-dimensional space of symmetric tensors at a point.

We now calculate each term.

### 2.1 $T_1$

$$\begin{aligned}T_1 &= \frac{1}{2}\mathrm{Tr}(M_1\mathbb{I}+M_P\mathbb{P})\\ &= \frac{1}{2}\frac{1}{(4\pi)^2}\int d^4x\sqrt{g}\{Q_2[M_1]\mathrm{tr}A_0+Q_1[M_1]\mathrm{tr}A_1+Q_0[M_1]\mathrm{tr}A_2\\ &\quad +Q_2[M_P]\mathrm{tr}(\mathbb{P}A_0)+Q_1[M_P]\mathrm{tr}(\mathbb{P}A_1)+Q_0[M_P]\mathrm{tr}(\mathbb{P}A_2)\}. \end{aligned}\tag{2.11}$$

### 2.2 $T_2$

$$\begin{aligned}T_2 &= -\frac{1}{2}\mathrm{Tr}(M_1\mathbb{I}+M_P\mathbb{P})(G_1\mathbb{I}+G_P\mathbb{P})V_1\\ &= \frac{1}{2}\mathrm{Tr}\left(V_1W_2(\Delta)+V_1\mathbb{P}W_{2P}(\Delta)\right), \end{aligned}\tag{2.12}$$

where

$$W_2=-M_1G_1\ ;\qquad W_{2P}=-(M_1G_P+M_PG_1+M_PG_P)\ .$$

$$\begin{aligned}T_2 &= \frac{1}{2}\frac{1}{(4\pi)^2}\int d^4x\sqrt{g}\Big\{-\frac{1}{2}Q_3[W_2]\,\mathrm{tr}(S_{\mu\nu}V_1^{\mu\nu}A_0)-\frac{1}{2}Q_2[W_2]\,\mathrm{tr}(S_{\mu\nu}V_1^{\mu\nu}A_1)\\ &\quad +Q_2[W_2]\,\mathrm{tr}V_1^{\mu\nu}\overline{D_{(\mu}D_{\nu)}A_0}\\ &\quad -\frac{1}{2}Q_3[W_{2P}]\,\mathrm{tr}(\mathbb{P}S_{\mu\nu}V_1^{\mu\nu}A_0)-\frac{1}{2}Q_2[W_{2P}]\,\mathrm{tr}(\mathbb{P}S_{\mu\nu}V_1^{\mu\nu}A_1)\\ &\quad +Q_2[W_{2P}]\,\mathrm{tr}(\mathbb{P}V_1^{\mu\nu}\overline{D_{(\mu}D_{\nu)}A_0})\Big\}. \end{aligned}\tag{2.13}$$

### 2.3 $T_3$

$$
\begin{aligned}
T_3 &= \frac{1}{2}\mathrm{Tr}(M_1\mathbb{I} + M_P\mathbb{P})(G_1\mathbb{I} + G_P\mathbb{P})V_1(G_1\mathbb{I} + G_P\mathbb{P})V_1 \\
&= \frac{1}{2}\mathrm{Tr}(V_1V_1W_3(\Delta) + V_1V_1\mathbb{P}W_{3P}(\Delta) + V_1\mathbb{P}V_1\mathbb{P}W_{3PP}(\Delta)),
\end{aligned}
\tag{2.14}
$$

where

$$
\begin{aligned}
&W_3 = M_1G_1^2 \ ; \qquad W_{3P} = 2M_1G_1G_P + M_PG_1^2 + M_PG_1G_P \ ; \\
&W_{3PP} = M_1G_P^2 + M_PG_1G_P + M_PG_P^2 \ .
\end{aligned}
\tag{2.15}
$$

Up to terms of higher order in curvature, we can commute the derivatives in $V_1$ with functions of $\Delta$. However, the order of $V_1$ and $\mathbb{P}$ has to be maintained. It is enough to work at order zero in the heat kernel expansion.

$$
\begin{aligned}
T_3 &= \frac{1}{2}\frac{1}{(4\pi)^2}\int d^4x\sqrt{g}\Big\{\frac{3}{4}Q_4[W_3]\mathrm{tr}(S_{\mu\nu\rho\sigma}V_1^{\mu\nu}V_1^{\rho\sigma}A_0) + \frac{3}{4}Q_4[W_{3P}]\mathrm{tr}(S_{\mu\nu\rho\sigma}V_1^{\mu\nu}V_1^{\rho\sigma}\mathbb{P}A_0) \\
&\qquad + \frac{3}{4}Q_4[W_{3PP}]\mathrm{tr}(S_{\mu\nu\rho\sigma}V_1^{\mu\nu}\mathbb{P}V_1^{\rho\sigma}\mathbb{P}A_0)\Big\}.
\end{aligned}
\tag{2.16}
$$

### 2.4 $T_4$

$$
T_4 = -\frac{1}{2}\mathrm{Tr}(M_1\mathbb{I} + M_P\mathbb{P})(G_1\mathbb{I} + G_P\mathbb{P})U_2 = \frac{1}{2}\mathrm{Tr}(W_4U_2 + W_{14}\mathbb{P}U_2),
\tag{2.17}
$$

where

$$
W_4 = -M_1G_1 \ ; \qquad W_{4P} = -(M_1G_P + M_PG_1 + M_PG_P),
$$

$$
T_4 = \frac{1}{2}\frac{1}{(4\pi)^2}\int d^4x\sqrt{g}\{Q_2[W_4]\mathrm{tr}(U_2A_0) + Q_2[W_{4P}]\mathrm{tr}(U_2\mathbb{P}A_0)\}.
\tag{2.18}
$$

### 2.5 $T_5$

This is the same as the calculation of $T_2$, but since $V_0$ has no $R$, we have to go to order $R^2$ in the heat kernel expansion.

$$
\begin{aligned}
T_5 &= \frac{1}{2}\mathrm{Tr}(V_0M_1\mathbb{I} + V_0M_P\mathbb{P}) \\
&= \frac{1}{2}\frac{1}{(4\pi)^2}\int d^4x\sqrt{g}\Big\{-\frac{1}{2}Q_3[M_1]\mathrm{tr}(S_{\mu\nu}V_0^{\mu\nu}A_0) - \frac{1}{2}Q_2[M_1]\mathrm{tr}(S_{\mu\nu}V_0^{\mu\nu}A_1) + Q_2[M_1]\mathrm{tr}V_0^{\mu\nu}\overline{D_{(\mu}D_{\nu)}A_0} \\
&\qquad -\frac{1}{2}Q_1[M_1]\mathrm{tr}(S_{\mu\nu}V_0^{\mu\nu}A_2) + Q_1[M_1]\mathrm{tr}\left(V_0^{\mu\nu}\overline{D_{(\mu}D_{\nu)}A_1}\right) \\
&\qquad -\frac{1}{2}Q_3[M_P]\mathrm{tr}(\mathbb{P}S_{\mu\nu}V_0^{\mu\nu}A_0) - \frac{1}{2}Q_2[M_P]\mathrm{tr}(\mathbb{P}S_{\mu\nu}V_0^{\mu\nu}A_1) + Q_2[M_P]\mathrm{tr}(\mathbb{P}V_0^{\mu\nu}\overline{D_{(\mu}D_{\nu)}A_0}) \\
&\qquad -\frac{1}{2}Q_1[M_P]\mathrm{tr}(\mathbb{P}S_{\mu\nu}V_0^{\mu\nu}A_2) + Q_1[M_P]\mathrm{tr}\left(\mathbb{P}V_0^{\mu\nu}\overline{D_{(\mu}D_{\nu)}A_1}\right)\Big\} \ .
\end{aligned}
\tag{2.19}
$$

## 2.6 $T_6$

$$
\begin{aligned}
T_6 &= \frac{1}{2}\mathrm{Tr}(M_1\mathbb{I}+M_P\mathbb{P})\left[(G_1\mathbb{I}+G_P\mathbb{P})V_0(G_1\mathbb{I}+G_P\mathbb{P})V_1+(G_1\mathbb{I}+G_P\mathbb{P})V_1(G_1\mathbb{I}+G_P\mathbb{P})V_0\right] \\
&= \frac{1}{2}\mathrm{Tr}\left[(V_0V_1+V_1V_0)W_3(\Delta)+(V_0V_1+V_1V_0)\mathbb{P}W_{3P}(\Delta)+2V_0\mathbb{P}V_1\mathbb{P}W_{3PP}(\Delta)\right] \ , \qquad (2.20)
\end{aligned}
$$

where the functions $W$ are the same as for $T_3$. Up to terms of higher order in curvature, we can commute the derivatives in $V_1$ with functions of $\Delta$. However, the order of $V_1$ and $\mathbb{P}$ has to be maintained.

In order to apply the HK formulae, we have to completely symmetrize the four derivatives attached to $V_0V_1$. To this end, let us define a ten-index tensor $T$ and an eight-index tensor $Z$ by

$$
\nabla_\mu\nabla_\nu\nabla_\rho\nabla_\sigma h_{\alpha\beta} = \nabla_{(\mu}\nabla_\nu\nabla_\rho\nabla_{\sigma)}h_{\alpha\beta} + T_{\mu\nu\rho\sigma}{}^{\lambda\tau}{}_{\alpha\beta}{}^{\gamma\delta}\nabla_{(\lambda}\nabla_{\tau)}h_{\gamma\delta} + Z_{\mu\nu\rho\sigma\alpha\beta}{}^{\gamma\delta}h_{\gamma\delta}.
$$

$T$ is linear in curvature and $Z$ is quadratic in curvature. We can view $T_{\mu\nu\rho\sigma}{}^{\lambda\tau}$ as a six-index tensor with values in endomorphism of the space of symmetric two-tensors. Then, for example, keeping only terms up to order $R^2$ and neglecting as usual terms of the form $\nabla R$,

$$
\begin{aligned}
\frac{1}{2}\mathrm{Tr}\left(V_0V_1W_3(\Delta)\right) &= \frac{1}{2}\int ds\tilde{W}_3(s)\mathrm{Tr}\left(V_0^{\mu\nu}V_1^{\rho\sigma}\nabla_\mu\nabla_\nu\nabla_\rho\nabla_\sigma e^{-s\Delta}\right) \\
&= \frac{1}{2}\int ds\tilde{W}_3(s)\mathrm{Tr}\left(V_0^{\mu\nu}V_1^{\rho\sigma}\nabla_{(\mu}\nabla_\nu\nabla_\rho\nabla_{\sigma)}e^{-s\Delta}\right) \\
&\quad+\frac{1}{2}\int ds\tilde{W}_3(s)\mathrm{Tr}\left(V_0^{\mu\nu}V_1^{\rho\sigma}T_{\mu\nu\rho\sigma}{}^{\lambda\tau}\nabla_{(\lambda}\nabla_{\tau)}e^{-s\Delta}\right).
\end{aligned}
$$

The first term has to be expanded to order $R$ of the HK expansion, giving

$$
\begin{aligned}
&\frac{1}{2}\int ds\tilde{W}_3(s)\mathrm{Tr}\left(V_0^{\mu\nu}V_1^{\rho\sigma}H_{(\mu\nu\rho\sigma)}\right) \\
&= \frac{1}{2}\frac{1}{(4\pi)^2}\int d^4x\sqrt{g}\Big\{\frac{3}{4}Q_4[W_3]\mathrm{tr}(S_{\mu\nu\rho\sigma}V_0^{\mu\nu}V_1^{\rho\sigma}A_0) \\
&\quad+Q_3[W_3]\left(\frac{3}{4}\mathrm{tr}(S_{\mu\nu\rho\sigma}V_0^{\mu\nu}V_1^{\rho\sigma}A_1)-3\mathrm{tr}(V_0^{\mu\nu}V_1^{\rho\sigma}g_{(\mu\nu}\overline{D_\rho D_{\sigma)}A_0})\right)\Big\}. \qquad (2.21)
\end{aligned}
$$

For the second term we need only the leading term of the HK expansion

$$
\begin{aligned}
&\frac{1}{2}\int ds\tilde{W}_3(s)\mathrm{Tr}\left(V_0^{\mu\nu}V_1^{\rho\sigma}T_{\mu\nu\rho\sigma}{}^{\lambda\tau}H_{(\lambda\tau)}\right) \\
&= \frac{1}{2}\frac{1}{(4\pi)^2}\int d^4x\sqrt{g}\Big\{-\frac{1}{2}Q_3[W_3]\,\mathrm{tr}(V_0^{\mu\nu}V_1^{\rho\sigma}T_{\mu\nu\rho\sigma}{}^{\lambda}{}_{\lambda}A_0)\Big\}. \qquad (2.22)
\end{aligned}
$$

The terms involving $\mathbb{P}$ can be dealt with in the same way. A slight simplification comes from the fact that the traces do not depend on the order of $V_0$ and $V_1$. Altogether we have

$$
\begin{aligned}
T_6 &= \frac{1}{2}\frac{1}{(4\pi)^2}\int d^4x\sqrt{g}\Big\{\frac{3}{4}Q_4[W_3]\mathrm{tr}(2S_{\mu\nu\rho\sigma}V_0^{\mu\nu}V_1^{\rho\sigma}A_0) \\
&\quad+Q_3[W_3]\left[\frac{3}{4}\mathrm{tr}(2S_{\mu\nu\rho\sigma}V_0^{\mu\nu}V_1^{\rho\sigma}A_1)-3\mathrm{tr}(2V_0^{\mu\nu}V_1^{\rho\sigma}g_{(\mu\nu}\overline{D_\rho D_{\sigma)}A_0})\right] \\
&\quad-\frac{1}{2}Q_3[W_3]\,\mathrm{tr}(2V_0^{\mu\nu}V_1^{\rho\sigma}T_{\mu\nu\rho\sigma}{}^{\lambda}{}_{\lambda}A_0)
\end{aligned}
$$

$$+\frac{3}{4}Q_4[W_{3P}]\mathrm{tr}(S_{\mu\nu\rho\sigma}(V_0^{\mu\nu}V_1^{\rho\sigma}+V_1^{\mu\nu}V_0^{\rho\sigma})\mathbb{P}A_0)$$
$$+Q_3[W_{3P}]\left(\frac{3}{4}\mathrm{tr}(S_{\mu\nu\rho\sigma}(V_0^{\mu\nu}V_1^{\rho\sigma}+V_1^{\mu\nu}V_0^{\rho\sigma})\mathbb{P}A_1)-3\mathrm{tr}((V_0^{\mu\nu}V_1^{\rho\sigma}+V_1^{\mu\nu}V_0^{\rho\sigma})\mathbb{P}g_{(\mu\nu}\overline{D_\rho D_{\sigma)}A_0})\right)$$
$$-\frac{1}{2}Q_3[W_{3P}]\,\mathrm{tr}(2V_0^{\mu\nu}V_1^{\rho\sigma}\mathbb{P}T_{\mu\nu\rho\sigma}{}^{\lambda}{}_{\lambda}A_0)$$
$$+\frac{3}{4}Q_4[W_{3PP}]\mathrm{tr}(2S_{\mu\nu\rho\sigma}V_0^{\mu\nu}\mathbb{P}V_1^{\rho\sigma}\mathbb{P}A_0)$$
$$+Q_3[W_{3PP}]\left(\frac{3}{4}\mathrm{tr}(2S_{\mu\nu\rho\sigma}V_0^{\mu\nu}\mathbb{P}V_1^{\rho\sigma}\mathbb{P}A_1)-3\mathrm{tr}(2V_0^{\mu\nu}\mathbb{P}V_1^{\rho\sigma}\mathbb{P}g_{(\mu\nu}\overline{D_\rho D_{\sigma)}A_0})\right)$$
$$-\frac{1}{2}Q_3[W_{3PP}]\,\mathrm{tr}(2V_0^{\mu\nu}\mathbb{P}V_1^{\rho\sigma}\mathbb{P}T_{\mu\nu\rho\sigma}{}^{\lambda}{}_{\lambda}A_0)\Big\}. \quad (2.23)$$

Note that

$$g_{(\mu\nu}\overline{D_\rho D_{\sigma)}A_0}=\frac{1}{6}g_{(\mu\nu}R_{\rho\sigma)}\ .$$

## 2.7 $T_7$

$$\begin{aligned}T_7 &= -\frac{1}{2}\mathrm{Tr}\left[M\left(GV_0GV_1GV_1+GV_1GV_0GV_0+GV_1GV_1GV_0\right)\right]\\ &= \frac{1}{2}\mathrm{Tr}[3(V_0V_1V_1)W_7(\Delta)+(V_0\mathbb{P}V_1V_1+V_0V_1\mathbb{P}V_1+V_0V_1V_1\mathbb{P})W_{7P1}(\Delta)\\ &\quad+(V_0\mathbb{P}V_1\mathbb{P}V_1+V_0\mathbb{P}V_1V_1\mathbb{P}+V_0V_1\mathbb{P}V_1\mathbb{P})W_{7P2}(\Delta)+3(V_0\mathbb{P}V_1\mathbb{P}V_1\mathbb{P})W_{7P3}(\Delta)]\ ,\end{aligned} \quad (2.24)$$

where

$$\begin{aligned}W_7 &= -3M_1G_1^3,\\ W_{7P1} &= -(3M_1G_1^2G_P+M_PG_1^2G_P+M_PG_1^3),\\ W_{7P2} &= -(3M_1G_1G_P^2+2M_PG_1^2G_P+2M_PG_1G_P^2),\\ W_{7P3} &= -3(M_1G_P^3+M_PG_1G_P^2+M_PG_P^3),\end{aligned} \quad (2.25)$$

and we have made use of the possibility to commute the $\nabla$'s with functions of $\Delta$, up to terms of higher order in curvature. (One can indeed check that if one could ignore all the $\mathbb{P}$'s, $W_7+3W_{7P1}+3W_{7P2}+W_{7P3}=-3(M_1+M_2)(G_1+G_2)^3$).

In order to apply the HK formulae, we have to completely symmetrize the six derivatives attached to $V_0V_1V_1$. This produces only terms of higher order in curvature. Then, to zeroth order in the HK expansion we have

$$\begin{aligned}T_7 &= \frac{1}{2}\frac{1}{(4\pi)^2}\int d^4x\sqrt{g}\Big\{-\frac{15}{8}Q_5[W_7]\,\mathrm{tr}(S_{\mu\nu\rho\sigma\lambda\tau}V_0^{\mu\nu}V_1^{\rho\sigma}V_1^{\lambda\tau}A_0)\\ &\quad-\frac{15}{8}Q_5[W_{7P1}]\,\mathrm{tr}(S_{\mu\nu\rho\sigma\lambda\tau}(V_0^{\mu\nu}\mathbb{P}V_1^{\rho\sigma}V_1^{\lambda\tau}+V_0^{\mu\nu}V_1^{\rho\sigma}\mathbb{P}V_1^{\lambda\tau}+V_0^{\mu\nu}V_1^{\rho\sigma}V_1^{\lambda\tau}\mathbb{P})A_0)\\ &\quad-\frac{15}{8}Q_5[W_{7P2}]\,\mathrm{tr}(S_{\mu\nu\rho\sigma\lambda\tau}(V_0^{\mu\nu}\mathbb{P}V_1^{\rho\sigma}\mathbb{P}V_1^{\lambda\tau}+V_0^{\mu\nu}\mathbb{P}V_1^{\rho\sigma}V_1^{\lambda\tau}\mathbb{P}+V_0^{\mu\nu}V_1^{\rho\sigma}\mathbb{P}V_1^{\lambda\tau}\mathbb{P})A_0)\\ &\quad-\frac{15}{8}Q_5[W_{7P3}]\,\mathrm{tr}(S_{\mu\nu\rho\sigma\lambda\tau}(V_0^{\mu\nu}\mathbb{P}V_1^{\rho\sigma}\mathbb{P}V_1^{\lambda\tau}\mathbb{P})A_0)\Big\}.\end{aligned} \quad (2.26)$$

### 2.8 $T_8$

$$
\begin{aligned}
T_8 &= \frac{1}{2}\mathrm{Tr}(M_1\mathbb{I}+M_P\mathbb{P})\left[(G_1\mathbb{I}+G_P\mathbb{P})V_0(G_1\mathbb{I}+G_P\mathbb{P})U_2+(G_1\mathbb{I}+G_P\mathbb{P})U_2(G_1\mathbb{I}+G_P\mathbb{P})V_0\right] \\
&= \frac{1}{2}\mathrm{Tr}\left[V_0U_2W_8(\Delta)+V_0U_2\mathbb{P}W_{8P}(\Delta)\right] \ , \qquad (2.27)
\end{aligned}
$$

where

$$
\begin{aligned}
W_8 &= 2M_1G_1^2, \\
W_{8P} &= 2(M_1(2G_1G_P+G_P^2)+M_P(G_1+G_P)^2). \qquad (2.28)
\end{aligned}
$$

In order to apply the HK formulae, we have to completely symmetrize the four derivatives attached to $V_0V_1$. This produces only terms of higher order in curvature, that can be neglected. To zeroth order in the HK expansion we have

$$
T_8=\frac{1}{2}\frac{1}{(4\pi)^2}\int d^4x\sqrt{g}\Big\{-\frac{1}{2}Q_3[W_8]\mathrm{tr}(S_{\mu\nu}V_0^{\mu\nu}U_2A_0)-\frac{1}{2}Q_3[W_{8P}]\mathrm{tr}(S_{\mu\nu}V_0^{\mu\nu}U_2\mathbb{P}A_0)\Big\}. \quad (2.29)
$$

### 2.9 $T_9$

$$
\begin{aligned}
T_9 &= -\frac{1}{2}\mathrm{Tr}(M_1\mathbb{I}+M_P\mathbb{P})(G_1\mathbb{I}+G_P\mathbb{P})U_1 \\
&= \frac{1}{2}\mathrm{Tr}\left[U_1W_9(\Delta)+U_1\mathbb{P}W_{9P}(\Delta)\right] \ , \qquad (2.30)
\end{aligned}
$$

where

$$
W_9=-M_1G_1 \ ; \qquad W_{9P}=-(M_1G_P+M_P(G_1+G_P)).
$$

Then to first order in the HK expansion

$$
\begin{aligned}
T_9 &= \frac{1}{2}\frac{1}{(4\pi)^2}\int d^4x\sqrt{g}\Big\{Q_2[W_9]\mathrm{tr}(U_1A_0)+Q_1[W_9]\mathrm{tr}(U_1A_1) \\
&\qquad +Q_2[W_9]\mathrm{tr}(U_1\mathbb{P}A_0)+Q_1[W_9]\mathrm{tr}(U_1\mathbb{P}A_1)\Big\}. \qquad (2.31)
\end{aligned}
$$

### 2.10 $T_{10}$

$$
\begin{aligned}
T_{10} &= \frac{1}{2}\mathrm{Tr}(M_1\mathbb{I}+M_P\mathbb{P})\left[(G_1\mathbb{I}+G_P\mathbb{P})V_1(G_1\mathbb{I}+G_P\mathbb{P})U_1+(G_1\mathbb{I}+G_P\mathbb{P})U_1(G_1\mathbb{I}+G_P\mathbb{P})V_1\right] \\
&= \frac{1}{2}\mathrm{Tr}\left[V_1U_1W_8(\Delta)+V_1U_1\mathbb{P}W_{8P}(\Delta)\right] \ , \qquad (2.32)
\end{aligned}
$$

where the $W$ functions are the same as for $T_8$. To zeroth order in the HK expansion we find

$$
T_{10}=\frac{1}{2}\frac{1}{(4\pi)^2}\int d^4x\sqrt{g}\Big\{-\frac{1}{2}Q_3[W_8]\mathrm{tr}(S_{\mu\nu}V_1^{\mu\nu}U_1A_0)-\frac{1}{2}Q_3[W_{8P}]\mathrm{tr}(S_{\mu\nu}V_1^{\mu\nu}U_1\mathbb{P}A_0)\Big\}. \quad (2.33)
$$

One can put these formulae into computer and derive the FRGE.

## 3 Graviton sector expanded to first order in $\Lambda$

The denominator in the first term $T^{\rm grav}$ in (1.1) contains nonminimal operator ($V$ and $U$). In the old approach, the nonminimal operators are all expanded. For comparison, we may also derive the FRGE in this scheme, by expanding the nonminimal operators as

$$
\begin{aligned}
T^{\rm grav} \;=\;& \frac{1}{2}{\rm Tr}\left[\frac{\partial_t R_k(\Delta^2)+\eta_K R_k(\Delta^2)}{P_k(\Delta^2)}\left(1-\frac{1}{P_k(\Delta^2)}(U+V)+\frac{1}{P_k^2(\Delta^2)}\Big\{U^2+(UV+VU)+V^2\Big\}\right.\right.\\
&\left.\left.+\frac{1}{P_k(\Delta^2)}\left[V,\frac{1}{P_k(\Delta^2)}\right](U+V)\;-\frac{1}{P_k^3(\Delta^2)}\left(UV^2+VUV+V^2U+V^2\right)\right)\right], \qquad (3.1)
\end{aligned}
$$

to quadratic order in the curvature, where $V\equiv V_{\mu\nu}\bar\nabla^\mu\bar\nabla^\nu$. We keep all terms up to order $Z_N$ and $\bar R^2$ (including $Z_N\bar R^2$ and $Z_N\Lambda\bar R$), but keep only first order in the cosmological constant, anticipating its FP value would be small. We can neglect the commutator term (first term in the second line) in the above to this order.

First let us concentrate on the first term in (3.1):

$$
\frac{1}{2}{\rm Tr}\frac{\partial_t R_k(\Delta^2)+\eta_K R_k(\Delta^2)}{P_k(\Delta^2)}.
$$

Calling $\tilde W$ the Laplace transform of $W$, we have for a second order differential operator $\Delta$ in four dimensions:

$$
\begin{aligned}
{\rm Tr}[W(\Delta)] &= \sum_n W(\lambda_n)=\sum_n\int_0^\infty ds\, e^{-\lambda_n s}\tilde W(s)=\int_0^\infty ds\,\tilde W(s)\,{\rm Tr}\,e^{-s\Delta}\\
&=\frac{1}{(4\pi)^2}\sum_{n=0}^\infty B_{2n}(\Delta)\int_0^\infty ds\,\tilde W(s)s^{n-2}=\frac{1}{(4\pi)^2}\sum_{n=0}^\infty B_{2n}(\Delta)\,Q_{2-n}(W), \qquad (3.2)
\end{aligned}
$$

where $B_{2n}=\int d^4x\sqrt{\bar g}\,{\rm tr}b_{2n}(x,x)$ are the coefficients appearing in the expansion of the trace of the heat kernel.

**Heat kernel for spin 2**

From [2] we have the heat kernel, to the necessary order, and at coincident points,

$$
{\rm Tr}\,e^{-s\Delta}=\frac{1}{(4\pi)^2}\left[\frac{1}{s^2}+\frac{1}{s}\frac{\bar R}{6}+\frac{\bar R^2}{72}-\frac{1}{180}(\bar R_{\mu\nu}^2-\bar R_{\mu\nu\alpha\beta}^2)+\frac{1}{12}\Omega_{\mu\nu}^2\right], \qquad (3.3)
$$

$$
\begin{aligned}
\bar\nabla_{(\mu}\bar\nabla_{\nu)}e^{-s\Delta} =\;& \frac{1}{(4\pi)^2}\mathbf{1}\left[-\frac{1}{2}\frac{1}{s^3}\bar g_{\mu\nu}-\frac{1}{12}\frac{1}{s^2}(\bar R\bar g_{\mu\nu}-2\bar R_{\mu\nu})\right.\\
&-\frac{1}{2s}\Big\{\left(\frac{1}{72}\bar R^2-\frac{1}{180}\bar R_{\alpha\beta}^2+\frac{1}{180}\bar R_{\alpha\beta\gamma\delta}^2+\frac{1}{12}\Omega_{\alpha\beta}^2\right)\bar g_{\mu\nu}-\frac{1}{18}\bar R\bar R_{\mu\nu}+\frac{2}{45}\bar R_{\mu\rho}\bar R_\nu{}^\rho\\
&\left.-\frac{1}{45}\bar R_{\rho\lambda}\bar R_\mu{}^\rho{}_\nu{}^\lambda-\frac{1}{45}\bar R_{\mu\alpha\beta\gamma}\bar R_\nu{}^{\alpha\beta\gamma}-\frac{1}{3}\Omega_{\alpha\mu}\Omega^\alpha{}_\nu\Big\}+\dots\right]. \qquad (3.4)
\end{aligned}
$$

$$
\bar\nabla_{(\mu}\bar\nabla_\nu\bar\nabla_\alpha\bar\nabla_{\beta)}e^{-s\Delta}=\frac{1}{(4\pi)^2}\left[\frac{3}{4s^4}\bar g_{(\mu\nu}\bar g_{\alpha\beta)}\mathbf{1}+\frac{1}{s^3}\left(\frac{1}{8}\bar g_{(\mu\nu}\bar g_{\alpha\beta)}\bar R-\frac{1}{2}\bar g_{(\mu\nu}\bar R_{\alpha\beta)}\right)+\dots\right]. \qquad (3.5)
$$

$$
\bar\nabla_{(\mu}\bar\nabla_\nu\bar\nabla_\rho\bar\nabla_\lambda\bar\nabla_\sigma\bar\nabla_{\tau)}e^{-s\Delta}=\frac{1}{(4\pi)^2}\frac{-15}{8s^5}\bar g_{(\mu\nu}\bar g_{\rho\lambda}\bar g_{\sigma\tau)}+\dots\;. \qquad (3.6)
$$

We define the $Q$-functionals (for $m>0$) by

$$Q^l_m(W)=\int_0^\infty ds\,\tilde W(s)s^{-m}=\frac{1}{\Gamma(m)}\int_0^\infty dz z^{m-1}W(z). \tag{3.7}$$

With the cutoff (1.9), the functionals that we need are

$$Q^l_m\left[\frac{\partial_t P_k+\eta_K R_k(z)}{P_k^\ell}\right]=k^{2(m-2\ell+2)}\left[\frac{4}{\Gamma(m+1)}+\frac{2\eta_K}{(m+2)\Gamma(m+1)}\right]. \tag{3.8}$$

Using these formulae, we calculate each terms as follows up to order $Z_N$ and $R^2$:

$$\begin{aligned}\frac{1}{2}\mathrm{Tr}\frac{\partial_t R_k(z)+\eta_K R_k(z)}{P_k(z)} &= \frac{1}{2}\int\frac{d^4x}{(4\pi)^2}\sqrt{g}\,\mathrm{tr}\left[Q^1_2\mathbf{1}+\frac{\bar R}{6}Q^1_1+\left(\frac{\bar R^2}{72}-\frac{1}{180}(\bar R^2_{\mu\nu}-\bar R^2_{\mu\nu\alpha\beta})+\frac{1}{12}\Omega^2_{\mu\nu}\right)Q^1_0\right]\\ &= \frac{1}{(4\pi)^2}\int d^4x\sqrt{g}\,\mathrm{tr}\left[k^4\left(1+\frac{\eta_1}{4}+\frac{\eta_P}{4}\mathbb{P}\right)+\frac{\bar R}{3}k^2\left(1+\frac{1}{6}\eta_1+\frac{1}{6}\eta_P\mathbb{P}\right)\right.\\ &\quad\left.+4\left(1+\frac{1}{4}\eta_1+\frac{1}{4}\eta_P\mathbb{P}\right)\left(\frac{1}{72}\bar R^2-\frac{1}{180}\bar R^2_{\alpha\beta}+\frac{1}{180}\bar R^2_{\alpha\beta\gamma\delta}+\frac{1}{12}\Omega^2_{\alpha\beta}\right)\right].\end{aligned} \tag{3.9}$$

**Linear in $U$:**

$$\begin{aligned}-\frac{1}{2}\mathrm{Tr}\left[U\frac{\partial_t R_k+\eta_K R_k}{P_k^2}\right] &= -\frac{1}{(4\pi)^2}\int d^4x\sqrt{g}\ \mathrm{tr}\left[\left(1+\frac{\eta_1}{8}+\frac{\eta_P}{8}\mathbb{P}\right)U+k^{-2}\frac{R}{3}\left(1+\frac{\eta_1}{6}+\frac{\eta_P}{6}\mathbb{P}\right)U\right.\\ &\quad\left.+\frac{k^{-4}}{2}(4+\eta_1+\eta_P\mathbb{P})\Big(\frac{1}{72}\bar R^2-\frac{1}{180}\bar R^2_{\alpha\beta}+\frac{1}{180}\bar R^2_{\alpha\beta\gamma\delta}+\frac{1}{12}\Omega^2_{\mu\nu}\Big)U\right],\end{aligned} \tag{3.10}$$

**Linear in $V$:**

$$\begin{aligned}&-\frac{1}{2}\mathrm{Tr}\left[\frac{\partial_t P_k+\eta_K R_k}{P_k^2}V^{\mu\nu}\bar\nabla_\mu\bar\nabla_\nu\right]\\ &=\frac{1}{(4\pi)^2}\int d^4x\sqrt{g}\ \mathrm{tr}\left[\frac{k^2}{6}\left(1+\frac{\eta_1}{10}+\frac{\eta_P}{10}\mathbb{P}\right)V^\mu_\mu+\left(1+\frac{\eta_1}{8}+\frac{\eta_P}{8}\mathbb{P}\right)\left(\frac{1}{12}\bar R V^\mu_\mu-\frac{1}{6}\bar R_{\mu\nu}V^{\mu\nu}\right)\right.\\ &\quad+k^{-2}\Big(1+\frac{\eta_1}{6}+\frac{\eta_P}{6}\mathbb{P}\Big)\Big\{\Big(\frac{1}{72}\bar R^2-\frac{1}{180}\bar R^2_{\alpha\beta}+\frac{1}{180}\bar R^2_{\alpha\beta\gamma\delta}+\frac{1}{12}\Omega^2_{\alpha\beta}\Big)V^\mu_\mu-\frac{1}{18}\bar R\bar R_{\mu\nu}V^{\mu\nu}\\ &\quad\left.+\frac{2}{45}\bar R_{\mu\rho}\bar R_\nu{}^\rho V^{\mu\nu}-\frac{1}{45}\bar R_{\rho\lambda}\bar R_\mu{}^\rho{}_\nu{}^\lambda V^{\mu\nu}-\frac{1}{45}\bar R_{\mu\rho\lambda\sigma}\bar R_\nu{}^{\rho\lambda\sigma}V^{\mu\nu}-\frac{1}{3}\Omega_{\rho\mu}\Omega^\rho{}_\nu V^{\mu\nu}\Big\}\right].\end{aligned} \tag{3.11}$$

**Quadratic term in $U$:**

$$\frac{1}{2}\mathrm{Tr}\left[U^2\frac{\partial_t P_k+\eta_K R_k}{P_k^3}\right]=\int\frac{d^4x}{(4\pi)^2}\sqrt{g}\ k^{-4}\mathrm{tr}\left[\left(1+\frac{\eta_1}{8}+\frac{\eta_P}{8}\mathbb{P}\right)U^2\right]. \tag{3.12}$$

**Terms containing $UV$:**

$$\begin{aligned}\frac{1}{2}\mathrm{Tr}\left[\frac{\partial_t P_k+\eta_K R_k}{P_k^3}2UV_{\mu\nu}\bar\nabla^\mu\bar\nabla^\nu\right] &= -\int\frac{d^4x}{(4\pi)^2}\sqrt{g}\,\mathrm{tr}\left[\frac{k^{-2}}{3}\left(1+\frac{\eta_1}{10}+\frac{\eta_P}{10}\mathbb{P}\right)UV^\mu_\mu\right.\\ &\quad\left.+\frac{k^{-4}}{3}\left(1+\frac{\eta_1}{8}+\frac{\eta_P}{8}\mathbb{P}\right)(RUV^\mu_\mu-2UV_{\mu\nu}\bar R^{\mu\nu})\right].\end{aligned} \tag{3.13}$$

**Quadratic terms in $V$:**

$$\frac{1}{2}\mathrm{Tr}\left[\frac{\partial_t P_k+\eta_K R_k}{P_k^3}V^{\mu\nu}V^{\alpha\beta}\bar\nabla_\mu\bar\nabla_\nu\bar\nabla_\alpha\bar\nabla_\beta\right] \tag{3.14}$$

To evaluate this, we need

$$\Big(\bar\nabla_\alpha\bar\nabla_\beta\bar\nabla_\gamma\bar\nabla_\delta\Big)^{\mu\nu}{}_{\rho\lambda} = \Big(\bar\nabla_{(\alpha}\bar\nabla_\beta\bar\nabla_\gamma\bar\nabla_{\delta)}\Big)^{\mu\nu}{}_{\rho\lambda} - \Big[\Big(R_{\beta\alpha}{}^{(\mu}{}_\rho\bar\nabla_\gamma\bar\nabla_\delta + R_{\gamma\alpha}{}^{(\mu}{}_\rho\bar\nabla_\beta\bar\nabla_\delta + R_{\delta\alpha}{}^{(\mu}{}_\rho\bar\nabla_\beta\bar\nabla_\gamma$$
$$+R_{\gamma\beta}{}^{(\mu}{}_\rho\bar\nabla_\alpha\bar\nabla_\delta + R_{\delta\beta}{}^{(\mu}{}_\rho\bar\nabla_\alpha\bar\nabla_\gamma + R_{\delta\gamma}{}^{(\mu}{}_\rho\bar\nabla_\alpha\bar\nabla_\beta\Big)\delta^{\nu)}_\lambda$$
$$+\Big(\frac{1}{3}R_{\gamma(\beta\alpha)\sigma}\bar\nabla^\sigma\bar\nabla_\delta + \frac{1}{2}R_{\gamma\sigma\beta\alpha}\bar\nabla^\sigma\bar\nabla_\delta + \frac{1}{3}R_{\delta(\beta\alpha)\sigma}\bar\nabla^\sigma\bar\nabla_\gamma + \frac{1}{2}R_{\delta\sigma\beta\alpha}\bar\nabla^\sigma\bar\nabla_\gamma$$
$$-\frac{1}{3}R_{\delta\gamma\sigma(\beta}\bar\nabla^\sigma\bar\nabla_{\alpha)} + \frac{1}{3}R_{\gamma\sigma\delta(\beta}\bar\nabla^\sigma\bar\nabla_{\alpha)} + R_{\delta\sigma\gamma(\beta}\bar\nabla^\sigma\bar\nabla_{\alpha)}\Big)\delta^{\mu\nu}{}_{\rho\lambda}\Big] + O(R^2). \tag{3.15}$$

The terms quadratic in curvatures give qubic in curvature and we can drop them. The first term on the rhs of (3.15) gives

$$\int \frac{d^4x}{(4\pi)^2}\sqrt{g}\ \mathrm{tr}\Big[Q_4^3\frac{3}{4}V^{\mu\nu}V^{\alpha\beta}\bar g_{(\mu\nu}\bar g_{\alpha\beta)} + Q_3^3\left(\frac{1}{8}\bar g_{(\mu\nu}\bar g_{\alpha\beta)}\bar R - \frac{1}{2}\bar g_{(\mu\nu}\bar R_{\alpha\beta)}\right)V^{\mu\nu}V^{\alpha\beta}\Big]$$
$$= \int \frac{d^4x}{(4\pi)^2}\sqrt{g}\ \mathrm{tr}\Big[\Big(1+\frac{\eta_1}{12}+\frac{\eta_P}{12}\mathbb{P}\Big)\frac{1}{16}V^{\mu\nu}V^{\alpha\beta}\bar g_{(\mu\nu}\bar g_{\alpha\beta)}$$
$$+k^{-2}\Big(1+\frac{\eta_1}{10}+\frac{\eta_P}{10}\mathbb{P}\Big)\Big\{\frac{\bar R}{24}V^{\mu\nu}V^{\alpha\beta}\bar g_{(\mu\nu}\bar g_{\alpha\beta)} - \frac{1}{6}\bar g_{(\mu\nu}\bar R_{\alpha\beta)}V^{\mu\nu}V^{\alpha\beta}\Big\}\Big]. \tag{3.16}$$

For the two covariant derivative terms in (3.5), we find that only the leading term in the heat kernel (3.4) proportional to $\bar g_{\mu\nu}$ contributes. We define

$$(T_{\alpha\beta\gamma\delta})^{\mu\nu}{}_{\rho\lambda} = \Big(R_{\beta\alpha}{}^{(\mu}{}_\rho\bar g_{\gamma\delta} + R_{\gamma\alpha}{}^{(\mu}{}_\rho\bar g_{\beta\delta} + R_{\delta\alpha}{}^{(\mu}{}_\rho\bar g_{\beta\gamma} + R_{\gamma\beta}{}^{(\mu}{}_\rho\bar g_{\alpha\delta} + R_{\delta\beta}{}^{(\mu}{}_\rho\bar g_{\alpha\gamma} + R_{\delta\gamma}{}^{(\mu}{}_\rho\bar g_{\alpha\beta}\Big)\delta^{\nu)}_\lambda$$
$$+\Big(\frac{1}{3}R_{\gamma(\beta\alpha)\delta} + \frac{1}{2}R_{\gamma\delta\beta\alpha} + \frac{1}{3}R_{\delta(\beta\alpha)\gamma} + \frac{1}{2}R_{\delta\gamma\beta\alpha} + \frac{1}{3}R_{\gamma(\alpha|\delta|\beta)} + R_{\delta(\alpha|\gamma|\beta)}\Big)\delta^{\mu\nu}{}_{\rho\lambda}\Big]. \tag{3.17}$$

Using (3.4), we find

$$-\frac{1}{2}\mathrm{Tr}\left[\frac{\partial_t P_k + \eta_K R_k}{P_k^3}V^{\alpha\beta}V^{\gamma\delta}T_{\alpha\beta\gamma\delta}\right] = \int \frac{d^4x}{(4\pi)^2}\sqrt{\bar g}\frac{k^{-2}Z_N}{6}\mathrm{tr}\left[\Big(1+\frac{\eta_1}{10}+\frac{\eta_P}{10}\mathbb{P}\Big)V^{\mu\nu}V^{\alpha\beta}T_{\mu\nu\alpha\beta}\right]. \tag{3.18}$$

$O(UV^2)$ **term:**

$$-\frac{1}{2}\mathrm{Tr}\left[\frac{\partial_t P_k + \eta_K R_k}{P_k^4}(UV_{\mu\nu}V_{\rho\lambda} + V_{\mu\nu}UV_{\rho\lambda} + V_{\mu\nu}V_{\rho\lambda}U)\bar\nabla^\mu\bar\nabla^\nu\bar\nabla^\rho\bar\nabla^\lambda\right]$$
$$= -\frac{1}{(4\pi)^2}\int d^4x\sqrt{\bar g}\frac{k^{-4}}{16}\mathrm{tr}\left[\Big(1+\frac{\eta_1}{12}+\frac{\eta_P}{12}\mathbb{P}\Big)(UV_{\mu\nu}V_{\rho\lambda} + V_{\mu\nu}UV_{\rho\lambda} + V_{\mu\nu}V_{\rho\lambda}U)\bar g^{(\mu\nu}\bar g^{\rho\lambda)}\right]. \tag{3.19}$$

$V^3$ **terms:** Use the formula (3.6), and we find

$$-\frac{1}{2}\mathrm{Tr}\left[\frac{\partial_t P_k + \eta_K R_k}{P_k^4}V_{\mu\nu}V_{\rho\lambda}V_{\sigma\tau}\bar\nabla^\mu\bar\nabla^\nu\bar\nabla^\rho\bar\nabla^\lambda\bar\nabla^\sigma\bar\nabla^\tau\right]$$
$$= \frac{1}{(4\pi)^2}\int d^4x\sqrt{\bar g}\frac{k^{-2}}{32}\mathrm{tr}\left[\Big(1+\frac{\eta_1}{14}+\frac{\eta_P}{14}\mathbb{P}\Big)\bar g^{(\mu\nu}\bar g^{\rho\lambda}\bar g^{\sigma\tau)}V_{\mu\nu}V_{\rho\lambda}V_{\sigma\tau}\right]. \tag{3.20}$$

Collecting everything, and using $\mathrm{tr}(\mathbf{1}) = 10$ and $\mathrm{tr}(\mathbb{P}) = 1$, we have

$$
\begin{aligned}
T^{grav} = & \frac{1}{(4\pi)^2}\int d^4x\sqrt{g}\Bigg[\left(10+\frac{5\eta_1}{4}+\frac{\eta_P}{8}\right)k^4+\left(\frac{10}{3}+\frac{5\eta_1}{9}+\frac{\eta_P}{18}\right)k^2\bar{R} \\
& +\left(1+\frac{\eta_1}{4}\right)\left(\frac{5}{18}\bar{R}^2-\frac{1}{9}\bar{R}^2_{\mu\nu}-\frac{8}{9}\bar{R}^2_{\mu\nu\alpha\beta}\right)+\frac{\eta_P}{360}\left(\bar{R}^2_{\mu\nu\rho\sigma}-\bar{R}^2_{\mu\nu}+\frac{5}{2}\bar{R}^2\right) \\
& +\mathrm{tr}\Bigg\{-\left(1+\frac{\eta_1}{8}+\frac{\eta_P}{8}\mathbb{P}\right)U-k^{-2}\frac{R}{3}\left(1+\frac{\eta_1}{6}+\frac{\eta_P}{6}\mathbb{P}\right)U \\
& -2k^{-4}\left(1+\frac{\eta_1}{4}+\frac{\eta_P}{4}\mathbb{P}\right)\left(\frac{1}{72}R^2-\frac{1}{180}R^2_{\alpha\beta}+\frac{1}{180}R^2_{\alpha\beta\gamma\delta}+\frac{1}{12}\Omega^2_{\alpha\beta}\right)U \\
& +\frac{k^2}{6}\left(1+\frac{\eta_1}{10}+\frac{\eta_P}{10}\mathbb{P}\right)V^\mu_\mu-\frac{1}{12}\left(1+\frac{\eta_1}{8}+\frac{\eta_P}{8}\mathbb{P}\right)(2\bar{R}_{\mu\nu}V^{\mu\nu}-\bar{R}V^\mu_\mu) \\
& +k^{-2}\left(1+\frac{\eta_1}{6}+\frac{\eta_P}{6}\mathbb{P}\right)\Big\{\Big(\frac{1}{72}\bar{R}^2-\frac{1}{180}\bar{R}^2_{\alpha\beta}+\frac{1}{180}\bar{R}^2_{\alpha\beta\gamma\delta}+\frac{1}{12}\Omega^2_{\alpha\beta}\Big)V^\mu_\mu-\frac{1}{18}\bar{R}\bar{R}_{\mu\nu}V^{\mu\nu} \\
& +\frac{2}{45}\bar{R}_{\mu\rho}\bar{R}_\nu{}^\rho V^{\mu\nu}-\frac{1}{45}\bar{R}_{\rho\lambda}\bar{R}_\mu{}^\rho{}_\nu{}^\lambda V^{\mu\nu}-\frac{1}{45}\bar{R}_{\mu\rho\lambda\sigma}\bar{R}_\nu{}^{\rho\lambda\sigma}V^{\mu\nu}-\frac{1}{3}\Omega_{\rho\mu}\Omega^\rho{}_\nu V^{\mu\nu}\Big\} \\
& +k^{-4}\mathrm{tr}\left(1+\frac{\eta_1}{8}+\frac{\eta_P}{8}\mathbb{P}\right)U^2-\frac{k^{-2}}{3}\left(1+\frac{\eta_1}{10}+\frac{\eta_P}{10}\mathbb{P}\right)UV^\mu_\mu \\
& -\frac{k^{-4}}{6}\left(1+\frac{\eta_1}{8}+\frac{\eta_P}{8}\mathbb{P}\right)(RUV^\mu_\mu-2UV_{\mu\nu}\bar{R}^{\mu\nu})+\left(1+\frac{\eta_1}{12}+\frac{\eta_P}{12}\mathbb{P}\right)\left(\frac{1}{48}V^\mu_\mu V^\nu_\nu+\frac{1}{24}V_{\mu\nu}V^{\mu\nu}\right) \\
& +\frac{k^{-2}}{6}\left(1+\frac{\eta_1}{10}+\frac{\eta_P}{10}\mathbb{P}\right)V^{\mu\nu}V^{\alpha\beta}T_{\mu\nu\alpha\beta}+k^{-2}\left(1+\frac{\eta_1}{10}+\frac{\eta_P}{10}\mathbb{P}\right)\Big\{\frac{\bar{R}}{72}(V^\mu_\mu V^\nu_\nu+2V_{\mu\nu}V^{\mu\nu}) \\
& -\frac{1}{18}(V^\mu_\mu V_{\nu\rho}\bar{R}^{\nu\rho}+2V_{\mu\nu}V^{\mu\rho}\bar{R}^\nu{}_\rho)\Big\}+\frac{k^{-2}}{32}\left(1+\frac{\eta_1}{14}+\frac{\eta_P}{14}\mathbb{P}\right)\bar{g}^{(\mu\nu}\bar{g}^{\rho\lambda}\bar{g}^{\sigma\tau)}V_{\mu\nu}V_{\rho\lambda}V_{\sigma\tau} \\
& -\frac{k^{-4}}{16}\left(1+\frac{\eta_1}{12}+\frac{\eta_P}{12}\mathbb{P}\right)\bar{g}^{(\mu\nu}\bar{g}^{\rho\lambda)}\frac{1}{3}(UV_{\mu\nu}V_{\rho\lambda}+V_{\mu\nu}UV_{\rho\lambda}+V_{\mu\nu}V_{\rho\lambda}U)\Bigg\}\Bigg]. \qquad (3.21)
\end{aligned}
$$

We list the necessary traces.

**Traces**

Here we give the traces of $U$ and $V$ in four dimensions. It is important to realize that the indices are symmetrized in $(\mu,\nu), (\alpha,\beta)$ and $(\rho,\lambda)$ in making products. Using

$$(\Omega_{\mu\nu})_{\alpha\beta,\gamma\delta} = R_{\mu\nu\alpha\gamma}g_{\beta\delta}+R_{\mu\nu\beta\delta}g_{\alpha\gamma}, \qquad (3.22)$$

we have

$$
\begin{aligned}
\mathrm{tr}(\Omega^2_{\alpha\beta}) &= -6R^2_{\alpha\beta\gamma\delta}, \\
\mathrm{tr}(\Omega^2_{\alpha\beta}U) &= Z_N\Lambda\frac{12}{\beta+4\gamma}R^2_{\alpha\beta\gamma\delta}+O(Z_N^2,R^3), \\
\mathrm{tr}(\Omega^2_{\alpha\beta}V^\mu_\mu) &= Z_N\frac{12}{\beta+4\gamma}R^2_{\alpha\beta\gamma\delta}+O(Z_N^2,R^3), \\
\mathrm{tr}(\Omega_{\rho\mu}\Omega^\rho{}_\nu V^{\mu\nu}) &= -\frac{Z_N}{\beta+4\gamma}(4R^2_{\mu\nu}-3R^2_{\alpha\beta\gamma\delta})+O(Z_N^2,R^3), \qquad (3.23)
\end{aligned}
$$

and other traces with projector $\mathbb{P}$ all vanish.

**Terms linear in $U$:**

$$\mathrm{tr}\ U = \delta^{\mu\nu,\alpha\beta}U_{\mu\nu,\alpha\beta} = A_1\bar{R}^2_{\mu\nu\rho\lambda}+A_2\bar{R}^2_{\mu\nu}+A_3\bar{R}^2+A_4Z_N\bar{R}+A_5Z_N\Lambda, \qquad (3.24)$$

where

$$A_1 = 3, \quad A_2 = \frac{4(\alpha+\beta+3\gamma)}{\beta+4\gamma}, \quad A_3 = \frac{2\alpha+\beta+2\gamma}{\beta+4\gamma},$$
$$A_4 = \frac{3}{\beta+4\gamma}, \quad A_5 = -\frac{2(28\alpha+9\beta+8\gamma)}{(3\alpha+\beta+\gamma)(\beta+4\gamma)}. \tag{3.25}$$

$$\mathrm{tr}\ (\mathbb{P}U) = \frac{1}{4}\,\bar{g}^{\mu\nu}\bar{g}^{\alpha\beta}U_{\mu\nu,\alpha\beta} = E_1\bar{R}^2_{\mu\nu\rho\lambda} + E_2\bar{R}^2_{\mu\nu} + E_3\bar{R}^2 + E_4 Z_N\bar{R} + E_5 Z_N\Lambda, \tag{3.26}$$

where

$$E_1 = E_2 = E_3 = E_4 = 0, \quad E_5 = -\frac{2(\alpha-\gamma)}{(3\alpha+\beta+\gamma)(\beta+4\gamma)}. \tag{3.27}$$

**Terms linear in $V$:**

$$\mathrm{tr}\ (V^\rho_\rho) = B_1\bar{R} + B_2 Z_N, \tag{3.28}$$

where

$$B_1 = \frac{4(8\alpha-3\beta-20\gamma)}{\beta+4\gamma}, \quad B_2 = -\frac{6(10\alpha+3\beta+2\gamma)}{(3\alpha+\beta+\gamma)(\beta+4\gamma)}. \tag{3.29}$$

$$\mathrm{tr}\ (V^{\rho\lambda}\bar{R}_{\rho\lambda}) = C_6\bar{R}^2_{\mu\nu} + C_7\bar{R}^2 + C_3 Z_N\bar{R}, \tag{3.30}$$

where

$$C_6 = \frac{8(-\alpha+\gamma)}{\beta+4\gamma}, \quad C_7 = \frac{10\alpha-3\beta-22\gamma}{\beta+4\gamma}, \quad C_3 = -\frac{3(10\alpha+3\beta+2\gamma)}{2(3\alpha+\beta+\gamma)(\beta+4\gamma)}. \tag{3.31}$$

$$\mathrm{tr}\ (\mathbb{P}V^\mu_\mu) = \frac{1}{4}\,\bar{g}^{\mu\nu}\bar{g}^{\alpha\beta}(V^\lambda_\lambda)_{\mu\nu,\alpha\beta} = F_1\bar{R} + F_2 Z_N, \tag{3.32}$$

where

$$F_1 = -\frac{4(\alpha-\gamma)}{\beta+4\gamma}, \quad F_2 = -\frac{6(\alpha-\gamma)}{(3\alpha+\beta+\gamma)(\beta+4\gamma)}. \tag{3.33}$$

$$\mathrm{tr}\ (\mathbb{P}V_{\mu\nu}\bar{R}^{\mu\nu}) = \frac{1}{d}\,\bar{g}^{\mu\nu}\bar{g}^{\alpha\beta}(V_{\rho\lambda})_{\mu\nu,\alpha\beta}\bar{R}^{\rho\lambda} = G_1\bar{R}^2_{\mu\nu} + G_2\bar{R}^2 + G_3 Z_N\bar{R}, \tag{3.34}$$

where

$$G_1 = 0, \quad G_2 = \frac{-\alpha+\gamma}{\beta+4\gamma}, \quad G_3 = -\frac{3(\alpha-\gamma)}{2(3\alpha+\beta+\gamma)(\beta+4\gamma)}. \tag{3.35}$$

$$\begin{aligned}
\mathrm{tr}(\bar{R}_{\mu\rho}\bar{R}_{\nu}{}^{\rho}V^{\mu\nu}) &= -Z_N\frac{3(10\alpha+3\beta+2\gamma)}{2(3\alpha+\beta+\gamma)(\beta+4\gamma)}\bar{R}_{\mu\nu}\bar{R}^{\mu\nu}+\cdots,\\
\mathrm{tr}(\bar{R}_{\rho\lambda}\bar{R}_{\mu}{}^{\rho}{}_{\nu}{}^{\lambda}V^{\mu\nu}) &= -Z_N\frac{3(10\alpha+3\beta+2\gamma)}{2(3\alpha+\beta+\gamma)(\beta+4\gamma)}\bar{R}_{\mu\nu}\bar{R}^{\mu\nu}+\cdots,\\
\mathrm{tr}(\bar{R}_{\mu\rho\lambda\sigma}\bar{R}_{\nu}{}^{\rho\lambda\sigma}V^{\mu\nu}) &= -Z_N\frac{3(10\alpha+3\beta+2\gamma)}{2(3\alpha+\beta+\gamma)(\beta+4\gamma)}\bar{R}_{\mu\nu\rho\lambda}\bar{R}^{\mu\nu\rho\lambda}+\cdots,\\
\mathrm{tr}(\mathbb{P}\bar{R}_{\mu\rho}\bar{R}_{\nu}{}^{\rho}V^{\mu\nu}) &= Z_N\frac{3(\alpha-\gamma)}{2(3\alpha+\beta+\gamma)(\beta+4\gamma)}\bar{R}_{\mu\nu}\bar{R}^{\mu\nu}+\cdots,\\
\mathrm{tr}(\mathbb{P}\bar{R}_{\rho\lambda}\bar{R}_{\mu}{}^{\rho}{}_{\nu}{}^{\lambda}V^{\mu\nu}) &= Z_N\frac{3(\alpha-\gamma)}{2(3\alpha+\beta+\gamma)(\beta+4\gamma)}\bar{R}_{\mu\nu}\bar{R}^{\mu\nu}+\cdots,\\
\mathrm{tr}(\mathbb{P}\bar{R}_{\mu\rho\lambda\sigma}\bar{R}_{\nu}{}^{\rho\lambda\sigma}V^{\mu\nu}) &= Z_N\frac{3(\alpha-\gamma)}{2(3\alpha+\beta+\gamma)(\beta+4\gamma)}\bar{R}_{\mu\nu\rho\lambda}\bar{R}^{\mu\nu\rho\lambda}+\cdots. \qquad (3.36)
\end{aligned}$$

**Traces of $U^2, UV$ and $V^2$:**

$$\mathrm{tr}(U^2)=\delta^{\mu\nu,\alpha\beta}(U^2)_{\mu\nu,\alpha\beta}=\tilde{A}_1Z_N\Lambda\bar{R}^2_{\mu\nu\rho\lambda}+\tilde{A}_2Z_N\Lambda\bar{R}^2_{\mu\nu}+\tilde{A}_3Z_N\Lambda\bar{R}^2+\cdots, \qquad (3.37)$$

where

$$\tilde{A}_1=-\frac{12}{\beta+4\gamma},\quad \tilde{A}_2=-\frac{16(\alpha+\beta+3\gamma)}{(\beta+4\gamma)^2},\quad \tilde{A}_3=-\frac{4(2\alpha+\beta+2\gamma)}{(\beta+4\gamma)^2}. \qquad (3.38)$$

$$\mathrm{tr}(\mathbb{P}U^2)=\frac{1}{4}\bar{g}^{\mu\nu}\bar{g}^{\alpha\beta}(U^2)_{\mu\nu,\alpha\beta}=0. \qquad (3.39)$$

$$\begin{aligned}
\mathrm{tr}(UV^{\rho}_{\rho}) &= \delta^{\mu\nu,\alpha\beta}(UV^{\rho}_{\rho})_{\mu\nu,\alpha\beta}\\
&= \tilde{B}_1Z_N\bar{R}^2_{\mu\nu\rho\lambda}+\tilde{B}_2Z_N\bar{R}^2_{\mu\nu}+\tilde{B}_3Z_N\bar{R}^2+\tilde{B}_4Z_N\Lambda\bar{R}+\cdots, \qquad (3.40)
\end{aligned}$$

where

$$\begin{aligned}
\tilde{B}_1 &= -\frac{18}{\beta+4\gamma},\quad \tilde{B}_2=\frac{8(-\alpha+8\beta+33\gamma)}{(\beta+4\gamma)^2},\quad \tilde{B}_3=\frac{8\alpha-22\beta-96\gamma}{(\beta+4\gamma)^2},\\
\tilde{B}_4 &= \frac{8(-26\alpha^2+3\beta^2+52\alpha\gamma+24\beta\gamma+22\gamma^2)}{(3\alpha+\beta+\gamma)(\beta+4\gamma)^2}. \qquad (3.41)
\end{aligned}$$

$$\begin{aligned}
\mathrm{tr}(\mathbb{P}UV^{\rho}_{\rho}) &= \frac{1}{4}\bar{g}^{\mu\nu}\bar{g}^{\alpha\beta}(UV^{\rho}_{\rho})_{\mu\nu,\alpha\beta}\\
&= \tilde{D}_1Z_N\bar{R}^2_{\mu\nu\alpha\beta}+\tilde{D}_2Z_N\bar{R}^2_{\mu\nu}+\tilde{D}_3Z_N\bar{R}^2+\tilde{D}_4Z_N\Lambda\bar{R}+\cdots, \qquad (3.42)
\end{aligned}$$

where

$$\tilde{D}_1=\tilde{D}_2=\tilde{D}_3=0,\quad \tilde{D}_4=\frac{8(\alpha-\gamma)^2}{(3\alpha+\beta+\gamma)(\beta+4\gamma)^2}. \qquad (3.43)$$

$$\begin{aligned}
\mathrm{tr}\left[V^{\mu\nu}V^{\rho\lambda}T_{\mu\nu\rho\lambda}\right] &= -2Z_N\Big(\frac{168\alpha^2+72\alpha\beta+5\beta^2-48\alpha\gamma-32\beta\gamma-40\gamma^2}{(3\alpha+\beta+\gamma)(\beta+4\gamma)^2}R^2\\
&\quad +8\frac{6\alpha+11\beta+38\gamma}{(\beta+4\gamma)^2}R^2_{\mu\nu}\Big). \qquad (3.44)
\end{aligned}$$

$$\mathrm{tr}\left[\mathbb{P}V^{\mu\nu}V^{\rho\lambda}T_{\mu\nu\rho\lambda}\right]=2Z_N(\alpha-\gamma)\Big(-\frac{1}{3(3\alpha+\beta+\gamma)(\beta+4\gamma)}R^2+\frac{4}{3(\beta+4\gamma)^2}R^2_{\mu\nu}\Big). \quad (3.45)$$

$$\begin{aligned}\mathrm{tr}(UV_{\mu\nu}\bar{R}^{\mu\nu}) &= \frac{16(\alpha-\gamma)(3\alpha+\beta+\gamma)}{(3\alpha+\beta+\gamma)(\beta+4\gamma)^2}Z_N\Lambda\bar{R}^2_{\mu\nu}\\ &\quad -\frac{2(32\alpha^2-3\beta^2+2\alpha(\beta-28\gamma)-26\beta\gamma-24\gamma^2}{(3\alpha+\beta+\gamma)(\beta+4\gamma)^2}Z_N\Lambda\bar{R}^2+O(\bar{R}^3),\end{aligned} \quad (3.46)$$

and

$$\mathrm{tr}(\mathbb{P}UV_{\mu\nu}\bar{R}^{\mu\nu})=\frac{2(\alpha-\gamma)^2}{(3\alpha+\beta+\gamma)(\beta+4\gamma)^2}Z_N\Lambda\bar{R}^2+O(\bar{R}^3). \quad (3.47)$$

$$\frac{1}{48}\mathrm{tr}\ (V^\rho_\rho V^\lambda_\lambda)+\frac{1}{24}\mathrm{tr}\ (V_{\rho_\lambda}V^{\rho\lambda})=D_1\bar{R}^2_{\mu\nu\rho\lambda}+D_2\bar{R}^2_{\mu\nu}+D_3\bar{R}^2+D_4Z_N\bar{R}, \quad (3.48)$$

where

$$\begin{aligned}&D_1=6,\quad D_2=\frac{2(2\alpha^2+13\beta^2+102\beta\gamma+202\gamma^2+2\alpha(\beta+2\gamma))}{3(\beta+4\gamma)^2},\\ &D_3=\frac{64\alpha^2-7\beta^2+16\alpha(\beta-4\gamma)-72\beta\gamma-112\gamma^2}{6(\beta+4\gamma)^2},\quad D_4=-\frac{3(20\alpha^2+10\alpha\beta+\beta^2-2\beta\gamma-4\gamma^2)}{2(3\alpha+\beta+\gamma)(\beta+4\gamma)^2}.\end{aligned} \quad (3.49)$$

$$\frac{1}{48}\mathrm{tr}\ (\mathbb{P}V^\rho_\rho V^\lambda_\lambda)+\frac{1}{24}\mathrm{tr}\ (\mathbb{P}V_{\rho_\lambda}V^{\rho\lambda})=H_1\bar{R}^2_{\mu\nu\rho\lambda}+H_2\bar{R}^2_{\mu\nu}+H_3\bar{R}^2+H_4Z_N\bar{R}, \quad (3.50)$$

where

$$\begin{aligned}&H_1=0,\quad H_2=\frac{2(-\alpha+\gamma)(3\alpha+\beta+\gamma)}{(\beta+4\gamma)^2},\quad H_3=\frac{(4\alpha+\beta)(\alpha-\gamma)}{2(\beta+4\gamma)^2},\\ &H_4=\frac{3(\alpha-\gamma)^2}{2(3\alpha+\beta+\gamma)(\beta+4\gamma)^2}.\end{aligned} \quad (3.51)$$

$$\begin{aligned}\mathrm{tr}(V^\mu_\mu V_{\nu\rho}\bar{R}^{\nu\rho}) &= I_1Z_N\bar{R}^2_{\mu\nu}+I_2Z_N\bar{R}^2+\cdots,\\ \mathrm{tr}(V_{\mu\nu}V^{\mu\rho}\bar{R}^\nu{}_\rho) &= J_1Z_N\bar{R}^2_{\mu\nu}+J_2Z_N\bar{R}^2+\cdots,\\ \mathrm{tr}(\mathbb{P}V^\mu_\mu V_{\nu\rho}\bar{R}^{\nu\rho}) &= K_1Z_N\bar{R}^2_{\mu\nu}+K_2Z_N\bar{R}^2+\cdots,\\ \mathrm{tr}(\mathbb{P}V_{\mu\nu}V^{\mu\rho}\bar{R}^\nu{}_\rho) &= L_1Z_N\bar{R}^2_{\mu\nu}+L_2Z_N\bar{R}^2+\cdots,\end{aligned} \quad (3.52)$$

with

$$\begin{aligned}&I_1=-\frac{16(-2\alpha+3\beta+14\gamma)}{(\beta+4\gamma)^2},\quad I_2=\frac{4(-30\alpha^2+7\alpha\beta+6\beta^2+88\alpha\gamma+41\beta\gamma+38\gamma^2)}{(3\alpha+\beta+\gamma)(\beta+4\gamma)^2},\\ &J_1=-\frac{8(2\alpha+7\beta+26\gamma)}{(\beta+4\gamma)^2},\quad J_2=\frac{-120\alpha^2-44\alpha\beta-\beta^2+64\alpha\gamma+36\beta\gamma+40\gamma^2}{(3\alpha+\beta+\gamma)(\beta+4\gamma)^2},\\ &K_1=\frac{8(\alpha-\gamma)}{(\beta+4\gamma)^2},\quad K_2=\frac{2(3\alpha-\beta-7\gamma)(\alpha-\gamma)}{(3\alpha+\beta+\gamma)(\beta+4\gamma)^2},\\ &L_1=\frac{4(\alpha-\gamma)}{(\beta+4\gamma)^2},\quad L_2=\frac{-\alpha+\gamma}{(3\alpha+\beta+\gamma)(\beta+4\gamma)}.\end{aligned} \quad (3.53)$$

**Traces of $UV^2$ and $V^3$:**

$$\frac{1}{3}\mathrm{tr}\left[(UV_{\mu\nu}V_{\alpha\beta}+V_{\mu\nu}UV_{\alpha\beta}+V_{\mu\nu}V_{\alpha\beta}U)g^{(\mu\nu}g^{\alpha\beta)}\right]$$
$$=-16Z_N\Lambda\Big(\frac{168\alpha^3+94\alpha^2\beta-8\alpha\beta^2-7\beta^3-128\alpha^2\gamma-252\alpha\beta\gamma-76\beta^2\gamma-376\alpha\gamma^2-178\beta\gamma^2-112\gamma^3}{(3\alpha+\beta+\gamma)(\beta+4\gamma)^3}\bar{R}^2$$
$$+4\frac{8\alpha^2+5\alpha\beta+13\beta^2+4\alpha\gamma+99\beta\gamma+196\gamma^2}{(\beta+4\gamma)^3}\bar{R}^2_{\mu\nu}+\frac{36}{\beta+4\gamma}\bar{R}^2_{\mu\nu\alpha\beta}\Big) \tag{3.54}$$

$$\frac{1}{3}\mathrm{tr}\left[\mathbb{P}(UV_{\mu\nu}V_{\alpha\beta}+V_{\mu\nu}UV_{\alpha\beta}+V_{\mu\nu}V_{\alpha\beta}U)g^{(\mu\nu}g^{\alpha\beta)}\right]$$
$$=16Z_N(\alpha-\gamma)\Lambda\left(\frac{4(5\alpha+\beta-\gamma)}{(\beta+4\gamma)^3}\bar{R}^2_{\mu\nu}-\frac{18\alpha^2+8\alpha\beta+\beta^2-4\alpha\gamma+2\gamma^2}{(3\alpha+\beta+\gamma)(\beta+4\gamma)^3}\bar{R}^2\right). \tag{3.55}$$

$$\mathrm{tr}\left(\bar{g}^{(\mu\nu}\bar{g}^{\rho\lambda}\bar{g}^{\sigma\tau)}V_{\mu\nu}V_{\rho\lambda}V_{\sigma\tau}\right)=\frac{32Z_N}{5(\beta+4\gamma)^3}\Big(-26(\beta+4\gamma)(-2\alpha+\beta+6\gamma)\bar{R}^2_{\mu\nu}$$
$$+\frac{-360\alpha^3+17\beta^3-24\alpha^2(8\beta-13\gamma)+178\beta^2\gamma+416\beta\gamma^2+264\gamma^3+\alpha(26\beta^2+592\beta\gamma+872\gamma^2)}{3\alpha+\beta+\gamma}\bar{R}^2$$
$$-36(\beta+4\gamma)^2\bar{R}^2_{\mu\nu\alpha\beta})\Big). \tag{3.56}$$

$$\mathrm{tr}\left(\mathbb{P}\bar{g}^{(\mu\nu}\bar{g}^{\rho\lambda}\bar{g}^{\sigma\tau)}V_{\mu\nu}V_{\rho\lambda}V_{\sigma\tau}\right)=32Z_N(\alpha-\gamma)\Big(\frac{4(21\alpha^2+4\alpha\beta-\beta^2-26\alpha\gamma-12\beta\gamma-11\gamma^2)}{15(3\alpha+\beta+\gamma)(\beta+4\gamma)^3}\bar{R}^2_{\mu\nu}$$
$$+\frac{-48\alpha^2-4\alpha\beta+\beta^2+80\alpha\gamma+12\beta\gamma-16\gamma^2}{15(3\alpha+\beta+\gamma)(\beta+4\gamma)^3}\bar{R}^2\Big). \tag{3.57}$$

Plugging these into (3.21), we can obtain the FRGE and derive the beta functions.

# 4 Ghost contributions

Next we evaluate the ghost contributions. Both ghosts operators are of the form

$$\Delta\delta^\nu_\mu+\sigma\bar{\nabla}_\mu\bar{\nabla}^\nu+B^\nu_\mu, \tag{4.1}$$

where $\sigma=-\frac{1-2\omega}{2(1+\omega)}$ and $B^\nu_\mu=-\bar{R}^\nu_\mu$ for $\Delta_{gh}$, and $\sigma=\frac{1-2\omega}{3}$ and $B^\nu_\mu=+\bar{R}^\nu_\mu$ for $Y$. After adding a cutoff term $R_k(\Delta)$, this becomes

$$P_k(\Delta)\delta^\nu_\mu+\sigma\bar{\nabla}_\mu\bar{\nabla}^\nu+B^\nu_\mu\ . \tag{4.2}$$

In the flow equation one needs the inverse of this operator. Since we only need all traces to order $\bar{R}^2$, we can treat the Ricci term by expanding. So first we need the inverse of

$$\mathcal{P}^\nu_\mu=P_k(\Delta)\delta^\nu_\mu+\sigma\bar{\nabla}_\mu\bar{\nabla}^\nu. \tag{4.3}$$

This can be obtained as follows. We make an ansatz

$$(\mathcal{P}^{-1})^\nu_\mu=P_k(\Delta)^{-1}\delta^\nu_\mu+\bar{\nabla}_\mu\bar{\nabla}^\nu g(\Delta)\ , \tag{4.4}$$

where $g$ is some function to be determined. From

$$\delta^\rho_\mu = (\mathcal{P}^{-1})^\nu_\mu \mathcal{P}^\rho_\nu,$$

ignoring the commutators between covariant derivatives, one finds

$$g_0(\Delta) = -\frac{\sigma}{P_k(\Delta)(P_k(\Delta) - \sigma\Delta)}.$$

This amounts to keeping the lowest order terms in $R$. Therefore we define

$$(\mathcal{P}_0^{-1})^\nu_\mu = P_k(\Delta)^{-1}\delta^\nu_\mu - \bar{\nabla}_\mu \bar{\nabla}^\nu \frac{\sigma}{P_k(\Delta)(P_k(\Delta) - \sigma\Delta)} \ , \tag{4.5}$$

Now we compute

$$(\mathcal{P})^\nu_\mu (\mathcal{P}_0^{-1})^\rho_\nu = \left\{ \delta^\rho_\mu - \sigma\left([P_k, \bar{\nabla}_\mu \bar{\nabla}^\rho] + \sigma \bar{\nabla}_\mu [\bar{\nabla}^\rho, \Delta]\right) \frac{1}{P_k(\Delta)(P_k(\Delta) - \sigma\Delta)} \right\}. \tag{4.6}$$

Calling $1 - M_1$ the curly bracket, we have

$$\mathcal{P} = (1 - M_1)\mathcal{P}_0,$$

or

$$\mathcal{P}^{-1} = \mathcal{P}_0^{-1}(1 + M_1 + M_1^2 + \ldots). \tag{4.7}$$

Up to terms of higher order in curvature, this is the formula of Groh et al. [4].

## 4.1 Explicit calculation

What we have to calculate is

$$\mathrm{Tr}\left[\frac{1}{\mathcal{P} + B}(\dot{R}_k + \eta R_k)\right] = \mathrm{Tr}\left[\left(\frac{1}{\mathcal{P}} - \frac{1}{\mathcal{P}}B\frac{1}{\mathcal{P}} + \frac{1}{\mathcal{P}}B\frac{1}{\mathcal{P}}B\frac{1}{\mathcal{P}}\right)(\dot{R}_k + \eta R_k)\right]. \tag{4.8}$$

We will evaluate these terms to the second order in the curvature and we can ignore contributions from commutators in the terms of order $R^2$.

We have

$$(M_0)_{\mu\nu} = -\sigma \bar{\nabla}_\mu \bar{\nabla}_\nu, \tag{4.9}$$

$$\begin{aligned}
(M_1)_\mu{}^\nu A_\nu &= \sigma\left([P_k, \nabla_\mu \nabla^\nu] + \sigma \nabla_\mu [\nabla^\nu, \Delta]\right) A_\nu \\
&= \sigma\left(-[\nabla_\mu \nabla^\nu, \Delta] P_k'(\Delta) + \frac{1}{2}[[\nabla_\mu \nabla^\nu, \Delta], \Delta]] P_k''(\Delta) + \sigma \nabla_\mu [\nabla^\nu, \Delta]\right) A_\nu \\
&= \sigma\Bigg((-R_{\mu\rho}\nabla^\rho \nabla^\nu + R^\nu_\rho \nabla_\mu \nabla^\rho) P_k'(\Delta) + \Big((R^\nu_\rho R_{\mu\lambda} - 2R^\nu_\lambda R_{\mu\rho})\nabla^\lambda \nabla^\rho + R^{\lambda\zeta} R^\nu{}_{\lambda\rho\zeta} \nabla_\mu \nabla^\rho \\
&\quad + \frac{R_{\rho\lambda}}{2}(R^\lambda_\mu \nabla^\rho \nabla^\nu - R^{\nu\lambda}\nabla_\mu \nabla^\rho)\Big) P_k''(\Delta) - \sigma R^\nu_\rho \nabla_\mu \nabla^\rho\Bigg) A_\nu + O(R^3).
\end{aligned} \tag{4.10}$$

$$
\begin{aligned}
(M_1^2)_\mu{}^\nu A_\nu &= \sigma^2 \Bigg( (-R_{\mu\rho}\nabla^\rho\nabla^\nu + R^\nu_\rho \nabla_\mu \nabla^\rho) P_k'(\Delta) - \sigma R^\nu_\rho \nabla_\mu \nabla^\rho \Bigg) \\
&\quad \times \Bigg( (-R_{\nu\lambda}\nabla^\lambda\nabla^\sigma + R^\sigma_\lambda \nabla_\nu \nabla^\lambda) P_k'(\Delta) - \sigma R^\sigma_\lambda \nabla_\nu \nabla^\lambda \Bigg) A_\sigma \\
&= \sigma^2 \Bigg( R_{\mu\rho} R_{\nu\lambda} \nabla^\rho \nabla^\nu \nabla^\lambda \nabla^\sigma P_k'(\Delta)^2 - R_{\mu\rho} R^\sigma_\lambda \nabla^\rho \nabla^\nu \nabla_\nu \nabla^\lambda P_k'(\Delta)^2 \\
&\quad + \sigma R_{\mu\rho} R^\sigma_\lambda \nabla^\rho \nabla^\nu \nabla_\nu \nabla^\lambda P_k'(\Delta) - R^\nu_\rho R_{\nu\lambda} \nabla_\mu \nabla^\rho \nabla^\lambda \nabla^\sigma P_k'(\Delta)^2 \\
&\quad + R^\nu_\rho R^\sigma_\lambda \nabla_\mu \nabla^\rho \nabla_\nu \nabla^\lambda P_k'(\Delta)^2 - \sigma R^\nu_\rho R^\sigma_\lambda \nabla_\mu \nabla^\rho \nabla_\nu \nabla^\lambda P_k'(\Delta) + \sigma R^\nu_\rho R_{\nu\lambda} \nabla_\mu \nabla^\rho \nabla^\lambda \nabla^\sigma P_k'(\Delta) \\
&\quad - \sigma R^\nu_\rho R^\sigma_\lambda \nabla_\mu \nabla^\rho \nabla_\nu \nabla^\lambda P_k'(\Delta) + \sigma^2 R^\nu_\rho R^\sigma_\lambda \nabla_\mu \nabla^\rho \nabla_\nu \nabla^\lambda \Bigg) A_\sigma, \qquad (4.11)
\end{aligned}
$$

where we have used the formula

$$
\begin{aligned}
[\Delta, [\Delta, \nabla_\mu \nabla^\nu]] A_\nu &= 2 \Bigg( (R^\nu_\rho R_{\mu\lambda} - 2 R^\nu_\lambda R_{\mu\lambda}) \nabla^\lambda \nabla^\rho + R^{\lambda\zeta} R^\nu{}_{\lambda\rho\zeta} \nabla_\mu \nabla^\rho \\
&\quad + \frac{R_{\rho\lambda}}{2} (R^\lambda_\mu \nabla^\rho \nabla^\nu - R^{\nu\lambda} \nabla_\mu \nabla^\rho) \Bigg) A_\nu + O(R^3), \qquad (4.12)
\end{aligned}
$$

and

$$
\nabla_\mu [\nabla^\nu, \Delta] A_\nu = -R^\nu_\rho \nabla_\mu \nabla^\rho A_\nu. \qquad (4.13)
$$

We note that $M_1$ is at least of order $R$.

We choose $P_k(\Delta) \equiv \Delta + R_k(\Delta) = \Delta + (k^2 - \Delta)\theta(k^2 - \Delta)$. As a distribution

$$
\begin{aligned}
P_k'(\Delta) &= 0, \\
P_k''(\Delta) &= \theta'(k^2 - \Delta), \\
\dot{R}_k(\Delta) &= 2k^2 \theta(k^2 - \Delta), \\
R_k'(\Delta) &= -\theta(k^2 - \Delta), \\
\dot{R}_k'(\Delta) &= -2k^2 \theta'(k^2 - \Delta), \qquad (4.14)
\end{aligned}
$$

where prime is the derivative with respect to $\Delta$. For this cutoff, we have

$$
\begin{aligned}
(M_1)_{\mu\nu} &= -\sigma^2 \bar{R}_{\rho\nu} \bar{\nabla}_\mu \bar{\nabla}^\rho + \sigma \Big( (R^\nu_\rho R_{\mu\lambda} - 2 R^\nu_\lambda R_{\mu\rho}) \nabla^\lambda \nabla^\rho + R^{\lambda\zeta} R^\nu{}_{\lambda\rho\zeta} \nabla_\mu \nabla^\rho \\
&\quad + \frac{R_{\rho\lambda}}{2} (R^\lambda_\mu \nabla^\rho \nabla^\nu - R^{\nu\lambda} \nabla_\mu \nabla^\rho) \Big) \theta'(k^2 - z), \qquad (4.15)
\end{aligned}
$$

so that to second order in curvature we have

$$
\begin{aligned}
\frac{1}{\mathcal{P}} = \left( \frac{1}{P_k(\Delta)} + M_0 \frac{1}{P_k(\Delta)(P_k(\Delta) - \sigma\Delta)} \right) \Bigg[ 1 + M_1 \frac{1}{P_k(\Delta)(P_k(\Delta) - \sigma\Delta)} \\
+ \left( M_1 \frac{1}{P_k(\Delta)(P_k(\Delta) - \sigma\Delta)} \right)^2 + \cdots \Bigg]. \qquad (4.16)
\end{aligned}
$$

We have to be careful that $M_0$ and $M_1$ are not diagonal.

The first term contributes

$$
\begin{aligned}
\mathrm{Tr}\Bigg(\Bigg\{ & \frac{1}{P_k} + M_1 \frac{1}{P_k^2(P_k-\sigma\Delta)} + M_1^2 \frac{1}{P_k^3(P_k-\sigma\Delta)^2} + M_0 \frac{1}{P_k(P_k-\sigma\Delta)} \\
& + M_0 M_1 \frac{1}{P_k^2(P_k-\sigma\Delta)^2} + M_0 \left[\frac{1}{P_k(P_k-\sigma\Delta)}, M_1\right] \frac{1}{P_k(P_k-\sigma\Delta)} \\
& + M_0 M_1^2 \frac{1}{P_k^3(P_k-\sigma\Delta)^3} \Bigg\}(\dot{R}_k + \eta R_k)\Bigg), \qquad (4.17)
\end{aligned}
$$

where we have kept only terms quadratic in the curvature.

We need the heat kernel for spin 1 [2], which are summarized in sect. 4.2. We find for (4.17)

$$
\begin{aligned}
\mathrm{Tr}\left[\frac{\dot{R}_k+\eta R_k}{P_k}\right] &= \frac{1}{(4\pi)^2}\int d^4x\sqrt{g}\,\Bigg[4k^4 Q_2^0(W) + \frac{2}{3}\bar{R}k^2 Q_1^0(W) \\
&\qquad + \left(\frac{1}{18}\bar{R}^2 - \frac{1}{45}\bar{R}_{\mu\nu}^2 - \frac{11}{180}\bar{R}_{\mu\nu\alpha\beta}^2\right) Q_0^0(W)\Bigg], \\
\mathrm{Tr}\left[M_1 \frac{(\dot{R}_k+\eta R_k)}{P_k^2(P_k-\sigma\Delta)}\right] &= \frac{1}{(4\pi)^2}\int d^4x\sqrt{g}\sigma^2\left[\frac{1}{2}k^2\bar{R}Q_3^1(W) + \left(\frac{1}{12}\bar{R}^2 + \frac{1}{3}R_{\mu\nu}^2\right) Q_2^1(W)\right], \\
\mathrm{Tr}\left[\frac{M_1^2(\dot{R}_k+\eta R_k)}{P_k^3(P_k-\sigma\Delta)^2}\right] &= \frac{1}{(4\pi)^2}\int d^4x\sqrt{g}\,\sigma^4 \frac{2\bar{R}_{\mu\nu}^2+\bar{R}^2}{4} Q_4^2(W), \\
\mathrm{Tr}\left[\frac{M_0(\dot{R}_k+\eta R_k)}{P_k(P_k-\sigma\Delta)}\right] &= \frac{1}{(4\pi)^2}\int d^4x\sqrt{g}\sigma\left(2Q_3^1(W)k^4 + \frac{2}{3}k^2\bar{R}Q_2^1(W) + \frac{\bar{R}^2+\bar{R}_{\mu\nu}^2}{12}Q_1^1(W)\right) \\
\mathrm{Tr}\left[\frac{M_0M_1(\dot{R}_k+\eta R_k)}{P_k^2(P_k-\sigma\Delta)^2}\right] &= \frac{1}{(4\pi)^2}\int d^4x\sqrt{g}\Bigg[\sigma^3\left(\frac{3}{2}Q_4^2(W)k^2\bar{R} + \frac{\bar{R}^2+7\bar{R}_{\mu\nu}^2}{6}Q_3^2(W)\right) \\
&\qquad + \frac{\sigma^2}{24(1-\sigma)^2}(R^2 - 4R_{\mu\nu}R^{\mu\nu})\Bigg]. \qquad (4.18)
\end{aligned}
$$

In evaluating this last term, we have used (4.14), (4.10) and (4.35). Furthermore

$$
\begin{aligned}
\mathrm{Tr}\left[\frac{M_0M_1^2(\dot{R}_k+\eta R_k)}{P_k^3(P_k-\sigma\Delta)^3}\right] &= \frac{1}{(4\pi)^2}\int d^4x\sqrt{g}\,\sigma^5(2\bar{R}_{\mu\nu}^2+\bar{R}^2)Q_5^3(W), \\
\mathrm{Tr}\left(M_0\left[\frac{1}{P_k(P_k-\sigma\Delta)}, M_1\right]\frac{\dot{R}_k+\eta R_k}{P_k(P_k-\sigma\Delta)}\right) &= \frac{1}{(4\pi)^2}\int d^4x\sqrt{g}\,\sigma^4\left(\bar{R}_{\mu\nu}^2 - \frac{1}{4}\bar{R}^2\right)Q_4^3(W). \qquad (4.19)
\end{aligned}
$$

Here we have defined

$$
Q_m^l(W) = \frac{1}{\Gamma(m)}\int_0^1 dy y^{m-1}\frac{2+\eta(1-y)}{(1-\sigma y)^l}, \qquad (4.20)
$$

and in particular

$$
Q_m^0(W) = \frac{1}{\Gamma(m+1)}\left(2 + \frac{\eta}{m+1}\right). \qquad (4.21)
$$

The term linear in $B$ has contributions

$$
\begin{aligned}
&-\mathrm{Tr}\left(B\frac{1}{\mathcal{P}}(\dot{R}_k+\eta R_k)\frac{1}{\mathcal{P}}\right) = -\mathrm{Tr}\left(B\frac{1}{\mathcal{P}^2}(\dot{R}_k+\eta R_k)+B\frac{1}{\mathcal{P}}\left[(\dot{R}_k+\eta R_k),\frac{1}{\mathcal{P}}\right]\right)\\
&= -\mathrm{Tr}\Bigg[B\Big\{\frac{1}{P_k^2}+\frac{M_0^2}{P_k^2(P_k-\sigma\Delta)^2}+\frac{2M_1}{P_k^3(P_k-\sigma\Delta)}+\frac{2M_0}{P_k^2(P_k-\sigma\Delta)}+\frac{3M_0M_1+M_1M_0}{P_k^3(P_k-\sigma\Delta)^2}\\
&+\frac{M_0^2M_1+M_0M_1M_0}{P_k^3(P_k-\sigma\Delta)^3}+M_0\left[\frac{1}{P_k(P_k-\Delta\sigma)},M_0\right]\frac{(\dot{R}_k+\eta R_k)}{P_k(P_k-\Delta\sigma)}\Big\}(\dot{R}_k+\eta R_k)\\
&+B\Big\{[\Delta,M_0]\frac{\dot{R}_k'(\Delta)+\eta R_k'(\Delta)}{P_k(\Delta)^2(P_k(\Delta)-\sigma\Delta)}+M_0[\Delta,M_0]\frac{\dot{R}_k'(\Delta)+\eta R_k'(\Delta)}{P_k(\Delta)^2(P_k(\Delta)-\sigma\Delta)^2}\Big\}\Bigg], \qquad (4.22)
\end{aligned}
$$

where the last two terms come from commuting

$$
\begin{aligned}
[\dot{R}_k+\eta R_k,\mathcal{P}^{-1}] &= [\dot{R}_k+\eta R_k,M_0]\frac{1}{P_k(\Delta)(P_k(\Delta)-\sigma\Delta)}\\
&= [\Delta,M_0]\frac{\dot{R}_k'(\Delta)+\eta R_k'(\Delta)}{P_k(\Delta)^(P_k(\Delta)-\sigma\Delta)}. \qquad (4.23)
\end{aligned}
$$

We find for (4.22)

$$
\begin{aligned}
-\mathrm{Tr}\left(\frac{B(\dot{R}_k+\eta R_k)}{P_k^2}\right) &= -\frac{B^\mu_\mu}{(4\pi)^2}\int d^4x\sqrt{g}\left[k^2Q_2^0(W)+\frac{\bar{R}}{6}Q_1^0(W)\right],\\
-\mathrm{Tr}\left[\frac{BM_0^2(\dot{R}_k+\eta R_k)}{P_k^2(P_k-\sigma\Delta)^2}\right] &= -\frac{1}{(4\pi)^2}\int d^4x\sqrt{g}\,\sigma^2\Big[k^2\frac{3B^\mu_\mu}{2}Q_4^2(W)\\
&\quad+\left(\frac{1}{6}B^\mu_\mu R+\frac{7}{6}B^{\mu\nu}R_{\mu\nu}\right)Q_3^2(W)\Big],\\
-\mathrm{Tr}\left[\frac{2BM_1(\dot{R}_k+\eta R_k)}{P_k^3(P_k-\sigma\Delta)}\right] &= -\frac{1}{(4\pi)^2}\int d^4x\sqrt{g}\,\sigma^2B_{\mu\nu}\bar{R}^{\mu\nu}Q_3^1(W),\\
-\mathrm{Tr}\left[\frac{2BM_0(\dot{R}_k+\eta R_k)}{P_k^2(P_k-\sigma\Delta)}\right] &= -\frac{1}{(4\pi)^2}\int d^4x\sqrt{g}\,\sigma\Bigg[k^2B^\mu_\mu Q_3^1(W)\\
&\quad+\frac{B^\mu_\mu\bar{R}+4B_{\mu\nu}\bar{R}^{\mu\nu}}{6}Q_2^1(W)\Bigg],\\
-\mathrm{Tr}\left[\frac{3BM_0M_1(\dot{R}_k+\eta R_k)}{P_k^3(P_k-\sigma\Delta)^2}\right] &= -\frac{1}{(4\pi)^2}\int d^4x\sqrt{g}\,\sigma^3\,\frac{9}{2}B_{\mu\nu}\bar{R}^{\mu\nu}Q_4^2(W),\\
-\mathrm{Tr}\left[\frac{BM_1M_0(\dot{R}_k+\eta R_k)}{P_k^3(P_k-\sigma\Delta)^2}\right] &= -\frac{1}{(4\pi)^2}\int d^4x\sqrt{g}\,\sigma^3\,\frac{2B_{\mu\nu}\bar{R}^{\mu\nu}+B^\mu_\mu\bar{R}}{4}Q_4^2(W),\\
-\mathrm{Tr}\left[\frac{BM_0^2M_1(\dot{R}_k+\eta R_k)}{P_k^3(P_k-\sigma\Delta)^3}\right] &= -\frac{1}{(4\pi)^2}\int d^4x\sqrt{g}\,\sigma^46B_{\mu\nu}\bar{R}^{\mu\nu}Q_5^3(W),\\
-\mathrm{Tr}\left[\frac{BM_0M_1M_0(\dot{R}_k+\eta R_k)}{P_k^3(P_k-\sigma\Delta)^3}\right] &= -\frac{1}{(4\pi)^2}\int d^4x\sqrt{g}\,\sigma^4(2B_{\mu\nu}\bar{R}^{\mu\nu}+B^\mu_\mu\bar{R})Q_5^3(W),
\end{aligned}
$$

$$-\mathrm{Tr}\left[BM_0\left[\frac{1}{P_k(P_k-\Delta\sigma)},M_0\right]\frac{(\dot{R}_k+\eta R_k)}{P_k(P_k-\Delta\sigma)}\right] = -\frac{\sigma^3}{(4\pi)^2}\int d^4x\sqrt{g}\left(R_{\mu\nu}B^{\mu\nu}-\frac{1}{4}RB^\mu_\mu\right)Q^3_4(W),$$

$$-\mathrm{Tr}\left[B[\Delta,M_0]\frac{\dot{R}'_k+\eta R'_k}{P_k^2(P_k-\sigma\Delta)}\right] = 0,$$

$$\begin{aligned}-\mathrm{Tr}\left[BM_0[\Delta,M_0]\frac{\dot{R}'_k+\eta R'_k}{P_k^2(P_k-\sigma\Delta)^2}\right] &= -\frac{\sigma^2}{(4\pi)^2}\int d^4x\sqrt{g}(R_{\mu\nu}B^{\mu\nu}-\frac{1}{4}RB^\mu_\mu)Q^2_4\left[\frac{\dot{R}'_k+\eta R'_k}{P_k^2(P_k-\sigma\Delta)^2}\right]\\ &= -\frac{\sigma^2}{(4\pi)^2}\int d^4x\sqrt{g}\frac{1}{6}(R_{\mu\nu}B^{\mu\nu}-\frac{1}{4}RB^\mu_\mu)\\ &\quad\times\left(-\frac{2}{(1-\sigma)^2}-\eta\int_0^1 dy\frac{y^3}{(1-\sigma y)^2}\right). \qquad (4.24)\end{aligned}$$

Finally the terms quadratic in $B$ makes contribution

$$\mathrm{Tr}\left[\frac{B^2}{P_k^3}+\frac{3B^2M_0}{P_k^3(P_k-\sigma\Delta)}+\frac{B^2M_0^2+2BM_0BM_0}{P_k^3(P_k-\sigma\Delta)^2}+\frac{BM_0BM_0^2}{P_k^3(P_k-\sigma\Delta)^3}\Big\}(\dot{R}_k+\eta R_k)\right]. \qquad (4.25)$$

We find for (4.25)

$$\begin{aligned}\mathrm{Tr}\left(\frac{B^2(\dot{R}_k+\eta R_k)}{P_k^3}\right) &= \frac{1}{(4\pi)^2}\int d^4x\sqrt{g}\,B^2_{\mu\nu}Q^0_2(W),\\ \mathrm{Tr}\left[\frac{3B^2M_0(\dot{R}_k+\eta R_k)}{P_k^3(P_k-\sigma\Delta)}\right] &= \frac{1}{(4\pi)^2}\int d^4x\sqrt{g}\,\frac{3}{2}B^2_{\mu\nu}\sigma Q^1_3(W),\\ \mathrm{Tr}\left[\frac{B^2M_0^2(\dot{R}_k+\eta R_k)}{P_k^3(P_k-\sigma\Delta)^2}\right] &= \frac{1}{(4\pi)^2}\int d^4x\sqrt{g}\,B^2_{\mu\nu}\frac{3}{2}\sigma^2Q^2_4(W),\\ \mathrm{Tr}\left[\frac{2BM_0BM_0(\dot{R}_k+\eta R_k)}{P_k^3(P_k-\sigma\Delta)^2}\right] &= \frac{1}{(4\pi)^2}\int d^4x\sqrt{g}\,\frac{2B^2_{\mu\nu}+(B^\mu_\mu)^2}{2}\sigma^2Q^2_4(W),\\ \mathrm{Tr}\left[\frac{BM_0BM_0^2(\dot{R}_k+\eta R_k)}{P_k^3(P_k-\sigma\Delta)^3}\right] &= \frac{1}{(4\pi)^2}\int d^4x\sqrt{g}\,[2B^2_{\mu\nu}+(B^\mu_\mu)^2]\sigma^3Q^3_5(W). \qquad (4.26)\end{aligned}$$

Collecting (4.18), (4.19), (4.24), and (4.26), we get

$$\begin{aligned}&\frac{1}{(4\pi)^{d/2}}\int d^4x\sqrt{g}\Big[k^4\Big\{3-\frac{2}{\sigma}-\frac{2}{\sigma^2}\log(1-\sigma)+\eta_G\Big(\frac{1}{\sigma^2}-\frac{1}{2\sigma}+\frac{1}{2}+\frac{1-\sigma}{\sigma^3}\log(1-\sigma)\Big)\Big\}\\ &\quad+k^2\bar{R}\left\{1+\frac{1}{2}\psi-\frac{1}{3\sigma}\log(1-\sigma)-\frac{\eta_G}{12}\Big(\frac{1}{\sigma}-\frac{3}{2}+\frac{2\sigma+1}{\sigma^2}\log(1-\sigma)\Big)\right\}\\ &\quad-k^2B^\mu_\mu\Big\{\frac{3}{4}+\frac{1}{2\sigma(1-\sigma)}+\frac{1}{2\sigma^2}\log(1-\sigma)+\frac{\eta_G}{8}\Big(1-\frac{4}{\sigma^2}-2\frac{2-\sigma}{\sigma^3}\log(1-\sigma)\Big\}\\ &\quad-\frac{11}{90}\Big(1+\frac{\eta_G}{2}\Big)\bar{R}^2_{\mu\nu\rho\lambda}+\Big\{\frac{\psi^2}{12}+\frac{1}{6}\psi-\frac{2}{45}+\eta_G\Big(\frac{13}{90}+\frac{\psi}{8}+\frac{1}{6\sigma}\log(1-\sigma)\Big)\Big\}\bar{R}^2_{\mu\nu}\\ &\quad+\Big\{\frac{\psi^2}{24}+\frac{\psi}{6}+\frac{1}{9}-\frac{\eta_G}{12}\Big(\frac{1}{3}+\frac{1}{\sigma}\log(1-\sigma)\Big)\Big\}\bar{R}^2-\Big\{\frac{\psi^2}{6}+\frac{2}{3}\psi-\frac{\eta_G}{24}\Big(\frac{2}{\sigma}+1-2\psi\\ &\quad+\frac{2}{\sigma^2}\log(1-\sigma)\Big)\Big\}B_{\mu\nu}\bar{R}^{\mu\nu}-\Big\{\frac{\psi^2}{12}+\frac{\psi}{6}+\frac{1}{3}+\frac{\eta_G}{12}\Big(\frac{5}{4}+\frac{1}{2\sigma}+\frac{\psi}{2}+\frac{1}{2\sigma^2}\log(1-\sigma)\Big)\Big\}B^\mu_\mu\bar{R}\\ &\quad+\Big\{\frac{\psi^2}{12}+\frac{\psi}{2}+1-\frac{\eta_G}{12}\Big(\frac{2+\sigma}{2\sigma^2}-\frac{5}{3}-\frac{1}{2}\psi+\frac{1}{\sigma^3}\log(1-\sigma)\Big)\Big\}B^2_{\mu\nu}\\ &\quad+\frac{1}{24}\Big\{\psi^2-\eta_G\Big(\frac{3}{2}\psi+\frac{4}{3}+\frac{1}{\sigma}-\frac{2}{\sigma^2(1-\sigma)}-\frac{2}{\sigma^3}\log(1-\sigma)\Big)\Big\}(B^\mu_\mu)^2\Big], \qquad (4.27)\end{aligned}$$

where $\psi = \frac{\sigma}{1-\sigma}$, and $\eta_G$ is the anomalous dimension for the ghost. The result for $\eta_G = 0$ agrees with Ref. [4].

## 4.2 Heat kernel for vectors

Let's recall the identity

$$R_\mu{}^{\alpha\beta\gamma} R_{\nu\gamma\alpha\beta} = -\frac{1}{2} R_\mu{}^{\alpha\beta\gamma} R_{\nu\alpha\beta\gamma} \tag{4.28}$$

For vectors the curvature $F_{\mu\nu}$ is given by

$$(F_{\mu\nu})^\alpha{}_\beta = R^\alpha{}_{\beta\mu\nu} \tag{4.29}$$

We need some off diagonal heat kernel coefficients (at coincidence points and neglecting derivatives of curvature) for vectors

$$\begin{aligned}
(A_0)^\alpha{}_\beta &= \delta^\alpha_\beta \\
\nabla_{(\mu}\nabla_{\nu)}(A_0)^\alpha{}_\beta &= \frac{1}{6} R_{\mu\nu}\delta^\alpha_\beta \\
(A_1)^\alpha{}_\beta &= -E^\alpha_\beta + \frac{1}{6} R\delta^\alpha_\beta \\
\nabla_{(\mu}\nabla_{\nu)}(A_1)^\alpha{}_\beta &= -\frac{1}{6} R_{\mu\nu} E^\alpha{}_\beta + \frac{1}{12}(R^\alpha{}_{\gamma\rho\nu} R^\gamma{}_\beta{}^\rho{}_\mu + R^\alpha{}_{\gamma\rho\mu} R^\gamma{}_\beta{}^\rho{}_\nu) + \frac{1}{36}\delta^\alpha_\beta R R_{\mu\nu} \\
&\quad -\frac{1}{45} R_{\mu\rho} R^\rho{}_\nu \delta^\alpha{}_\beta + \frac{1}{90} R_{\rho\lambda} R^\rho{}_\nu{}^\lambda{}_\mu \delta^\alpha{}_\beta + \frac{1}{90} R^{\rho\sigma\lambda}{}_\mu R^{\rho\sigma\lambda}{}_\nu \delta^\alpha{}_\beta \\
A_2 &= \frac{1}{2} E^\alpha{}_\gamma E^\gamma{}_\beta - \frac{1}{6} R E^\alpha{}_\beta + \frac{1}{12} R^\alpha{}_{\gamma\mu\nu} R^\gamma{}_\beta{}^{\mu\nu} \\
&\quad + \frac{1}{72} R^2 \delta^\alpha_\beta - \frac{1}{180} R_{\mu\nu} R^{\mu\nu} \delta^\alpha_\beta + \frac{1}{180} R_{\mu\nu\rho\lambda} R^{\mu\nu\rho\lambda} \delta^\alpha_\beta
\end{aligned} \tag{4.30}$$

Then we have

$$(e^{-s\Delta})^{\mu\lambda} = \frac{1}{(4\pi)^2}\left[\frac{1}{s^2}\bar g^{\mu\lambda} + \frac{1}{6s}\bar R \bar g^{\mu\lambda} + \frac{1}{12}\bar R^\mu{}_{\rho\alpha\beta} R^{\rho\lambda\alpha\beta} + \left(\frac{1}{72}\bar R^2 - \frac{1}{180}\bar R^2_{\mu\nu} + \frac{1}{180}\bar R^2_{\mu\nu\alpha\beta}\right)\bar g^{\mu\lambda}\right], \tag{4.31}$$

$$\begin{aligned}
\nabla_{(\mu}\nabla_{\nu)}(e^{-s(\Delta+E)})^{\sigma,\lambda} &= \frac{1}{(4\pi s)^2}\Bigg( -\frac{1}{2s} g_{\mu\nu}(A_0)^{\sigma,\lambda} - \frac{1}{2} g_{\mu\nu}(A_1)^{\sigma\lambda} + \nabla_{(\mu}\nabla_{\nu)}(A_0)^{\sigma\lambda} \\
&\quad -\frac{s}{2} g_{\mu\nu}(A_2)^{\sigma\lambda} + s\nabla_{(\mu}\nabla_{\nu)}(A_1)^{\sigma\lambda}\Bigg)
\end{aligned} \tag{4.32}$$

which leads to

$$\begin{aligned}
\nabla_\mu\nabla_\nu(e^{-s(\Delta+E)})^{\nu,\lambda} &= \left(\nabla_{(\mu}\nabla_{\nu)} + \frac{1}{2}[\nabla_\mu, \nabla_\nu]\right)(e^{-s(\Delta+E)})^{\nu,\lambda} \qquad (4.33) \\
&= \nabla_{(\mu}\nabla_{\nu)}(e^{-s(\Delta+E)})^{\nu,\lambda} + \frac{1}{2} R^\nu{}_{\rho\mu\nu}(e^{-s(\Delta+E)})^{\rho,\lambda} \\
&= \nabla_{(\mu}\nabla_{\nu)}(e^{-s(\Delta+E)})^{\nu,\lambda} - \frac{1}{2} R_{\mu\rho}(e^{-s(\Delta+E)})^{\rho,\lambda}
\end{aligned}$$

$$
\begin{aligned}
= \quad & \frac{1}{(4\pi s)^2}\Bigg[ -\frac{1}{2s}\delta^\lambda_\mu + \frac{1}{2}E^\lambda_\mu - \delta^\lambda_\mu \frac{1}{12}R + \frac{1}{6}R^\lambda{}_\mu + s\Big( -\frac{1}{4}E_{\mu\rho}E^{\rho\lambda} \\
& + \frac{1}{12}E_\mu{}^\lambda R - \frac{1}{24}R_{\mu\nu\alpha\beta}R^{\nu\lambda\alpha\beta} - \frac{1}{144}R^2\delta^\lambda_\mu + \frac{1}{360}R_{\alpha\beta}R^{\alpha\beta}\delta^\lambda_\mu \\
& - \frac{1}{360}R_{\rho\sigma\alpha\beta}R^{\rho\sigma\alpha\beta}\delta^\lambda_\mu - \frac{1}{6}R_{\mu\nu}E^{\nu\lambda} + \frac{1}{12}(R^\gamma{}_{\rho\alpha\mu}R^{\rho\lambda\alpha}{}_\gamma + R^\gamma{}_{\rho\alpha\gamma}R^{\rho\lambda\alpha}{}_\mu) \\
& + \frac{1}{36}RR^\lambda_\mu - \frac{1}{45}R_{\mu\rho}R^{\rho\lambda} + \frac{1}{90}R_{\alpha\beta}R^\alpha{}_\mu{}^{\beta\lambda} + \frac{1}{90}R^{\alpha\beta\gamma}{}_\mu R_{\alpha\beta\gamma}{}^\lambda\Big)\Bigg] \\
& + \frac{1}{(4\pi s)^2}(-\frac{1}{2}R^\lambda_\mu + \frac{1}{2}sR_{\mu\rho}E^{\rho\lambda} - s\frac{1}{12}RR^\lambda_\mu) \\
= \quad & \frac{1}{(4\pi s)^2}\Bigg[ -\frac{1}{2s}\delta^\lambda_\mu + \frac{1}{2}E^\lambda_\mu - \delta^\lambda_\mu \frac{1}{12}R - \frac{1}{3}R^\lambda{}_\mu + s\Big( -\frac{1}{4}E_{\mu\rho}E^{\rho\lambda} \\
& + \frac{1}{12}E_\mu{}^\lambda R - \frac{1}{144}R^2\delta^\lambda_\mu + \frac{1}{360}R_{\alpha\beta}R^{\alpha\beta}\delta^\lambda_\mu - \frac{1}{360}R_{\rho\sigma\alpha\beta}R^{\rho\sigma\alpha\beta}\delta^\lambda_\mu + \frac{1}{3}R_{\mu\nu}E^{\nu\lambda} \\
& - \frac{1}{18}RR^\lambda_\mu - \frac{1}{45}R_{\mu\rho}R^{\rho\lambda} - \frac{13}{180}R_{\alpha\beta}R^\alpha{}_\mu{}^{\beta\lambda} + \frac{1}{90}R^{\alpha\beta\gamma}{}_\mu R_{\alpha\beta\gamma}{}^\lambda\Big)\Bigg] \qquad (4.34)
\end{aligned}
$$

We also need

$$
\nabla_\mu\nabla_\nu(\Delta\, e^{-s\Delta})^{\nu,\lambda} \quad = \quad \frac{1}{(4\pi s)^2}\Bigg[ -\frac{3}{2}\delta^\lambda_\mu\frac{1}{s^2} - \delta^\lambda_\mu\frac{1}{6s}R - \frac{2}{3s}R^\lambda{}_\mu + \cdots \Bigg], \qquad (4.35)
$$

which is obtained by differentiating (4.34) with respect to $s$.

Furthermore, for symmetrized four and more derivative terms, we have

$$
\begin{aligned}
&\bar\nabla_{(\mu}\bar\nabla_\nu\bar\nabla_\rho\bar\nabla_{\lambda)}(e^{-s\Delta})^\lambda{}_\sigma = \frac{1}{(4\pi)^2}\left[\frac{3}{4s^4}\bar g_{(\mu\nu}\bar g_{\rho\sigma)} + \frac{1}{s^3}\left(\frac{1}{8}\bar R\bar g_{(\mu\nu}\bar g_{\rho\sigma)} - \frac{1}{2}\bar g_{(\mu\nu}\bar R_{\rho\sigma)}\right)\right], \\
&\bar\nabla_{(\mu}\bar\nabla_\nu\bar\nabla_\rho\bar\nabla_\lambda\bar\nabla_\sigma\bar\nabla_{\tau)}(e^{-s\Delta})^\tau{}_\alpha = \frac{1}{(4\pi)^2}\left(-\frac{15}{8}\right)\frac{1}{s^5}\bar g_{(\mu\nu}\bar g_{\rho\lambda}\bar g_{\sigma\alpha)}. \qquad (4.36)
\end{aligned}
$$

# References


[1] D. Benedetti, K. Groh, P. F. Machado and F. Saueressig, "The Universal RG Machine," JHEP **1106** (2011) 079 [arXiv:1012.3081 [hep-th]].

[2] K. Groh, F. Saueressig and O. Zanusso, "Off-diagonal heat-kernel expansion and its application to fields with differential constraints," arXiv:1112.4856 [math-ph].

[3] N. Ohta and R. Percacci, "Higher Derivative Gravity and Asymptotic Safety in Diverse Dimensions," Class. Quant. Grav. **31** (2014) 015024 [arXiv:1308.3398 [hep-th]].

[4] K. Groh, S. Rechenberger, F. Saueressig and O. Zanusso, "Higher Derivative Gravity from the Universal Renormalization Group Machine," PoS EPS **-HEP2011** (2011) 124 [arXiv:1111.1743 [hep-th]].
